# Supplementary material for: On Generative Agents in Recommendation
Source: arXiv:2310.10108 source file (2024-11-08)
Supplement: Supplementary file 1 [file 7_appendix.tex]

\appendix
\clearpage
\section{Related Works}
\subsection{LLM-empowered Generative Agents}
AI agents are artificial entities that sense their environment, make decisions, and take actions \cite{Survey_Fudan}. Human has long been pursuing intelligent agent to handle various task \cite{jennings1998roadmap, franklin1996agent, panait2005cooperative}.  Recently, with the remarkable capability of Large Language Model (LLM) demonstrated, a substantial body of research has emerged \cite{Survey_Renmin}. Generative Agent \cite{Generative_Agent} is a pioneer work that designs general agents equipped with memory, planning, and reflection abilities to simulate the human’s daily life. Building upon this universal framework, the following agent architecture can be bifurcated into task-oriented agents and simulation-oriented agents \cite{Survey_Fudan}.

The core objective of task-oriented agents is to execute predefined tasks established by humans \cite{Voyager, ChatDev, AutoGen, InteRecAgent, RecMind, RoCo}.  Within this category,  Voyager \cite{Voyager} integrates LLM into the Minecraft universe, endowing the in-game character with the capacity to effectively explore the virtual world. ChatDev \cite{ChatDev} introduces a novel agent collaboration paradigm in the domain of software development, harnessing group intelligence to streamline the development pipeline. AutoGen \cite{AutoGen} further extends this paradigm by defining more complex roles and facilitating multi-agent communication to tackle a diverse range of challenges.  In the realm of recommendation systems, RecMind \cite{RecMind} designs an LLM-powered autonomous recommender agent that possesses self-inspiring planning abilities and the capability to leverage external tools. InteRecAgent \cite{InteRecAgent} takes a step beyond by enhancing LLM-based agents with integrated components, yielding recommenders that are both explainable and conversational.

Simulation-oriented agents are geared towards replicating human behaviors in specific scenarios, thereby enabling the acquisition of valuable data and the exploration of social issues \cite{S3, Socially_alignment, RecAgent, WereWolf, Generative_Agent, AgentSims}. Among simulation-oriented agents, $S^{3}$ \cite{S3} leverages autonomous agents to simulate the dynamic evolution of public opinion on social platforms in response to trending social events. SANDBOX \cite{Socially_alignment} facilitates communication among a group of agents to address social issues thus providing ethically sound data for LLM fine-tuning. Differing from task-oriented agents in the field of recommendation, simulation-oriented agents seek to emulate user behaviors within recommender systems rather than focusing on the recommender. RecAgent \cite{RecAgent} attempts to integrate diverse user behaviors in recommendation environments, taking into account external social relationships. Focusing on simulating and evaluating user interactions with the recommenders, our framework Agent4Rec also falls into the category of simulation-oriented agents.

% In the realm of recommendation systems, there are few works available\cite{RecMind, InteRecAgent}. Among them, RecMind and InteRecAgent are task-oriented agents. RecMind \cite{RecMind} designs an LLM-powered autonomous recommender agent that possesses self-inspiring planning abilities and the capability to leverage external tools. InteRecAgent \cite{InteRecAgent} takes a step further by enhancing LLM-based agents with integrated components, yielding explainable and conversational recommender. Differing from the former works, simulation-oriented agents seek to emulate user behaviors within recommender systems rather than focusing on the recommender. RecAgent \cite{RecAgent} aims to simulate multi-type user behaviors in recommender system with external social relationships taken into consideration. Our framework Agent4Rec also falls into this category.

\subsection{Recommendation Simulator}
Recommendation simulator is a cornerstone in the field of recommendation systems \cite{reinforcement_survey_simulator, Feedback_loop, top_n_simulator, mindsim_simulator}. It diverges from conventional methods that rely on real-world user data, as it excels in replicating or simulating user interactions within recommender systems. This approach offers a cost-effective alternative to online environments and also presents a potential avenue for addressing prevalent challenges such as casual discovery and filter bubbles \cite{debias_simulator, adver_user_model_simulator}.
Early forays into recommendation simulators primarily serve as rich data sources for subsequent utilization, particularly in the realm of reinforcement learning \cite{Virtual-Taobao, RecSim, RecoGym}. For example, Virtual Taobao \cite{Virtual-Taobao} proposes a virtual environment based on real user interactions to simulate user behaviors on e-commerce platforms. RecSim \cite{RecSim} provides comprehensive toolkits for effectively simulating user behaviors in the setting of sequential recommendation. Also, RecoGym \cite{RecoGym} integrates both traditional recommendation algorithms and reinforcement learning framework, followed by evaluation with online and offline metrics. MINDSim \cite{mindsim_simulator} simulates user behaviors in a news website. But these traditional simulators all fall short in relatively simple rules, thus lacking flexibility and validity. Recently, LLM-empowered agents have demonstrated significant promise in approximating human-like intelligence, which showcases considerable potential for recommendation simulators \cite{Survey_Fudan, Survey_Renmin}. RecAgent \cite{RecAgent} makes the primary attempt to construct a recommendation platform to integrate diverse user behaviors involving movie-watching, chatting, posting, and searching. Instead of behavior integration, we set our sights on in-depth exploration to emulate and evaluate user interactions with both rule-based and algorithm-based recommenders in recommender systems.

\section{Agent4Rec}
\subsection{Agent Architecture}
\subsubsection{Profile Module}
% \subsubsection{Split of Social Traits.}
\textbf{Split of Social Traits.} 
\label{sec:app_social_traits} Utilizing the social traits defined in Section \ref{sec:method_profile} (\ie $T_{act}^{u}$, $T_{conf}^{u}$ and $T_{div}^{u}$), we categorize users into three groups within each trait based on the degree of intensity. Specifically, we allocate the social trait of activity to each user based on the ascending order of $T_{act}^{u}$ with a ratio of 6:3:1. Similarly, we assign the conformity trait and diversity trait in the same manner with the ratios of 1:2:1 and 1:1:1, respectively. We assign the same social traits for all users within the same group. 
This categorization is motivated by the long-tail distribution observed in user activity \cite{user_long_tail}, while the distributions of the other two traits are relatively normal. 
\textbf{User unique tastes generation.}
% \subsubsection{User unique tastes generation.} 
The prompts used for generating user unique tastes are illustrated in Figure \ref{fig:TasteGeneration}.
% \textbf{Unique Tastes}
% \subsubsection{Memory Module} \label{sec:app_memory}
\subsubsection{Memory Module} In Agent4Rec, our memory module consists of a vector store and a retriever. We apply FAISS \cite{FAISS} along with Openai embedding model \footnote{\url{www.openai.com}} as our vector store to store user memory units. And we apply Langchain \footnote{\url{www.langchain.com}} to implement our retriever, which enables us to retrieve memories based on relevant scores.
The prompts we used for user satisfaction reflection are listed in Figure \ref{fig:SatReflect}. 
\subsubsection{Action Module} \label{sec:app_action}
In Agent4Rec, agents will primarily take the following actions:
\begin{itemize}[leftmargin=*]
\item Reacting to recommended movie list, including, viewing, rating, and feeling generation
\item Deciding whether to exit the recommender system based on the level of satisfaction and level of fatigue.
\item Responding to the post-exit feeling interview.
\end{itemize}
The relevant prompts for agents making these actions are listed in Figure \ref{fig:ReactToItems}, \ref{fig:NextDecision}, and \ref{fig:InterviewCase}.
% Reflecting current satisfaction with the recommender system based on interaction history in the former pages
% \subsubsection{Generate movie profile including genre selection and summarization generation based on prior knowledge stored in LLM}

\subsection{Recommendation Environment} \label{sec:app_environment}
The prompts we used for generating movie summaries are listed in Figure \ref{fig:SummaryGeneration}.

\section{Experiments}\label{sec:experiment}
\subsection{Experiment Settings}
\subsubsection{Dataset}
% To evaluate the performance of our methods, 
We conduct all the experiments based on Movielens-1M \cite{MovieLens} dataset, which consists of 1,000,209 user-item rating interactions. We randomly sample 1,000 users to initialize agents, and divide the interaction history of each user into training, validation, and testing sets with a ratio of 4:3:3. 
To address the cold start problem, we remove movies from the testing and validation sets that do not appear in the training set.
% It is noted that our items pool only comprises movies rated by our sampled users. 
\subsubsection{Recommendation Strategy Settings}
In this study, five commonly used recommendation strategies in collaborative filtering are incorporated for recommending movies to agents. Both rule-based strategies (\ie random, most popular) and algorithm-based strategies (\ie MF, MultVAE, LightGCN) are employed in Agent4Rec.\\
For rule-bassed strategies, random denotes randomly recommending movies from the whole movie pool, while Pop denotes randomly recommending from 600 most popular movies.\\
For algorithm-based strategies, we optimize all methods with the Adam optimizer and set the embedding size as 64 for LightGCN and MF, the layer numbers of LightGCN by default at 2, the learning rate by default at 5e-4. For MultVAE, we adopt the original design \cite{MultVAE} of the [I → 600 → 200 → 600 → I] encoder-decoder structure, with $\beta$ at 0.2 and the total steps for annealing at 200,000.
If Recall@20 on the validation set does not increase for 20 successive evaluations, we adopt the early stop strategy to stop training.
\subsubsection{Platform Settings.} 
For all the experiments, we run Agent4Rec on a Linux server with a single NVIDIA RTX A5000 24GB GPU and a AMD EPYC 7543P 32-Core CPU. 
% The average cost for each round of simulation with a max exit page of 5 and a movie-per-page of 4 is around 16 dollars (\ie 0.016 dollars/user), affected by the number of pages each user browses. 
The average cost for the whole simulation of 1,000 agents, with four movies on one page and a max exit page of five, is around 16 dollars (\ie 0.016 dollars/user), affected by the number of pages each user browses. 
The simulation time depends on the TPM (tokens per minute) limitation of the OpenAI API key. With one single OpenAI API key of 350,000 TPM, the whole simulation of 1,000 agents takes 50 minutes.

\subsection{Social Traits Alignment} 
\label{sec:traits_appendix}
\begin{figure}[t]
	\centering
	\subcaptionbox{Activity\label{fig:bar_true_act}}{
	    \vspace{-6pt}
		\includegraphics[width=0.32\linewidth]{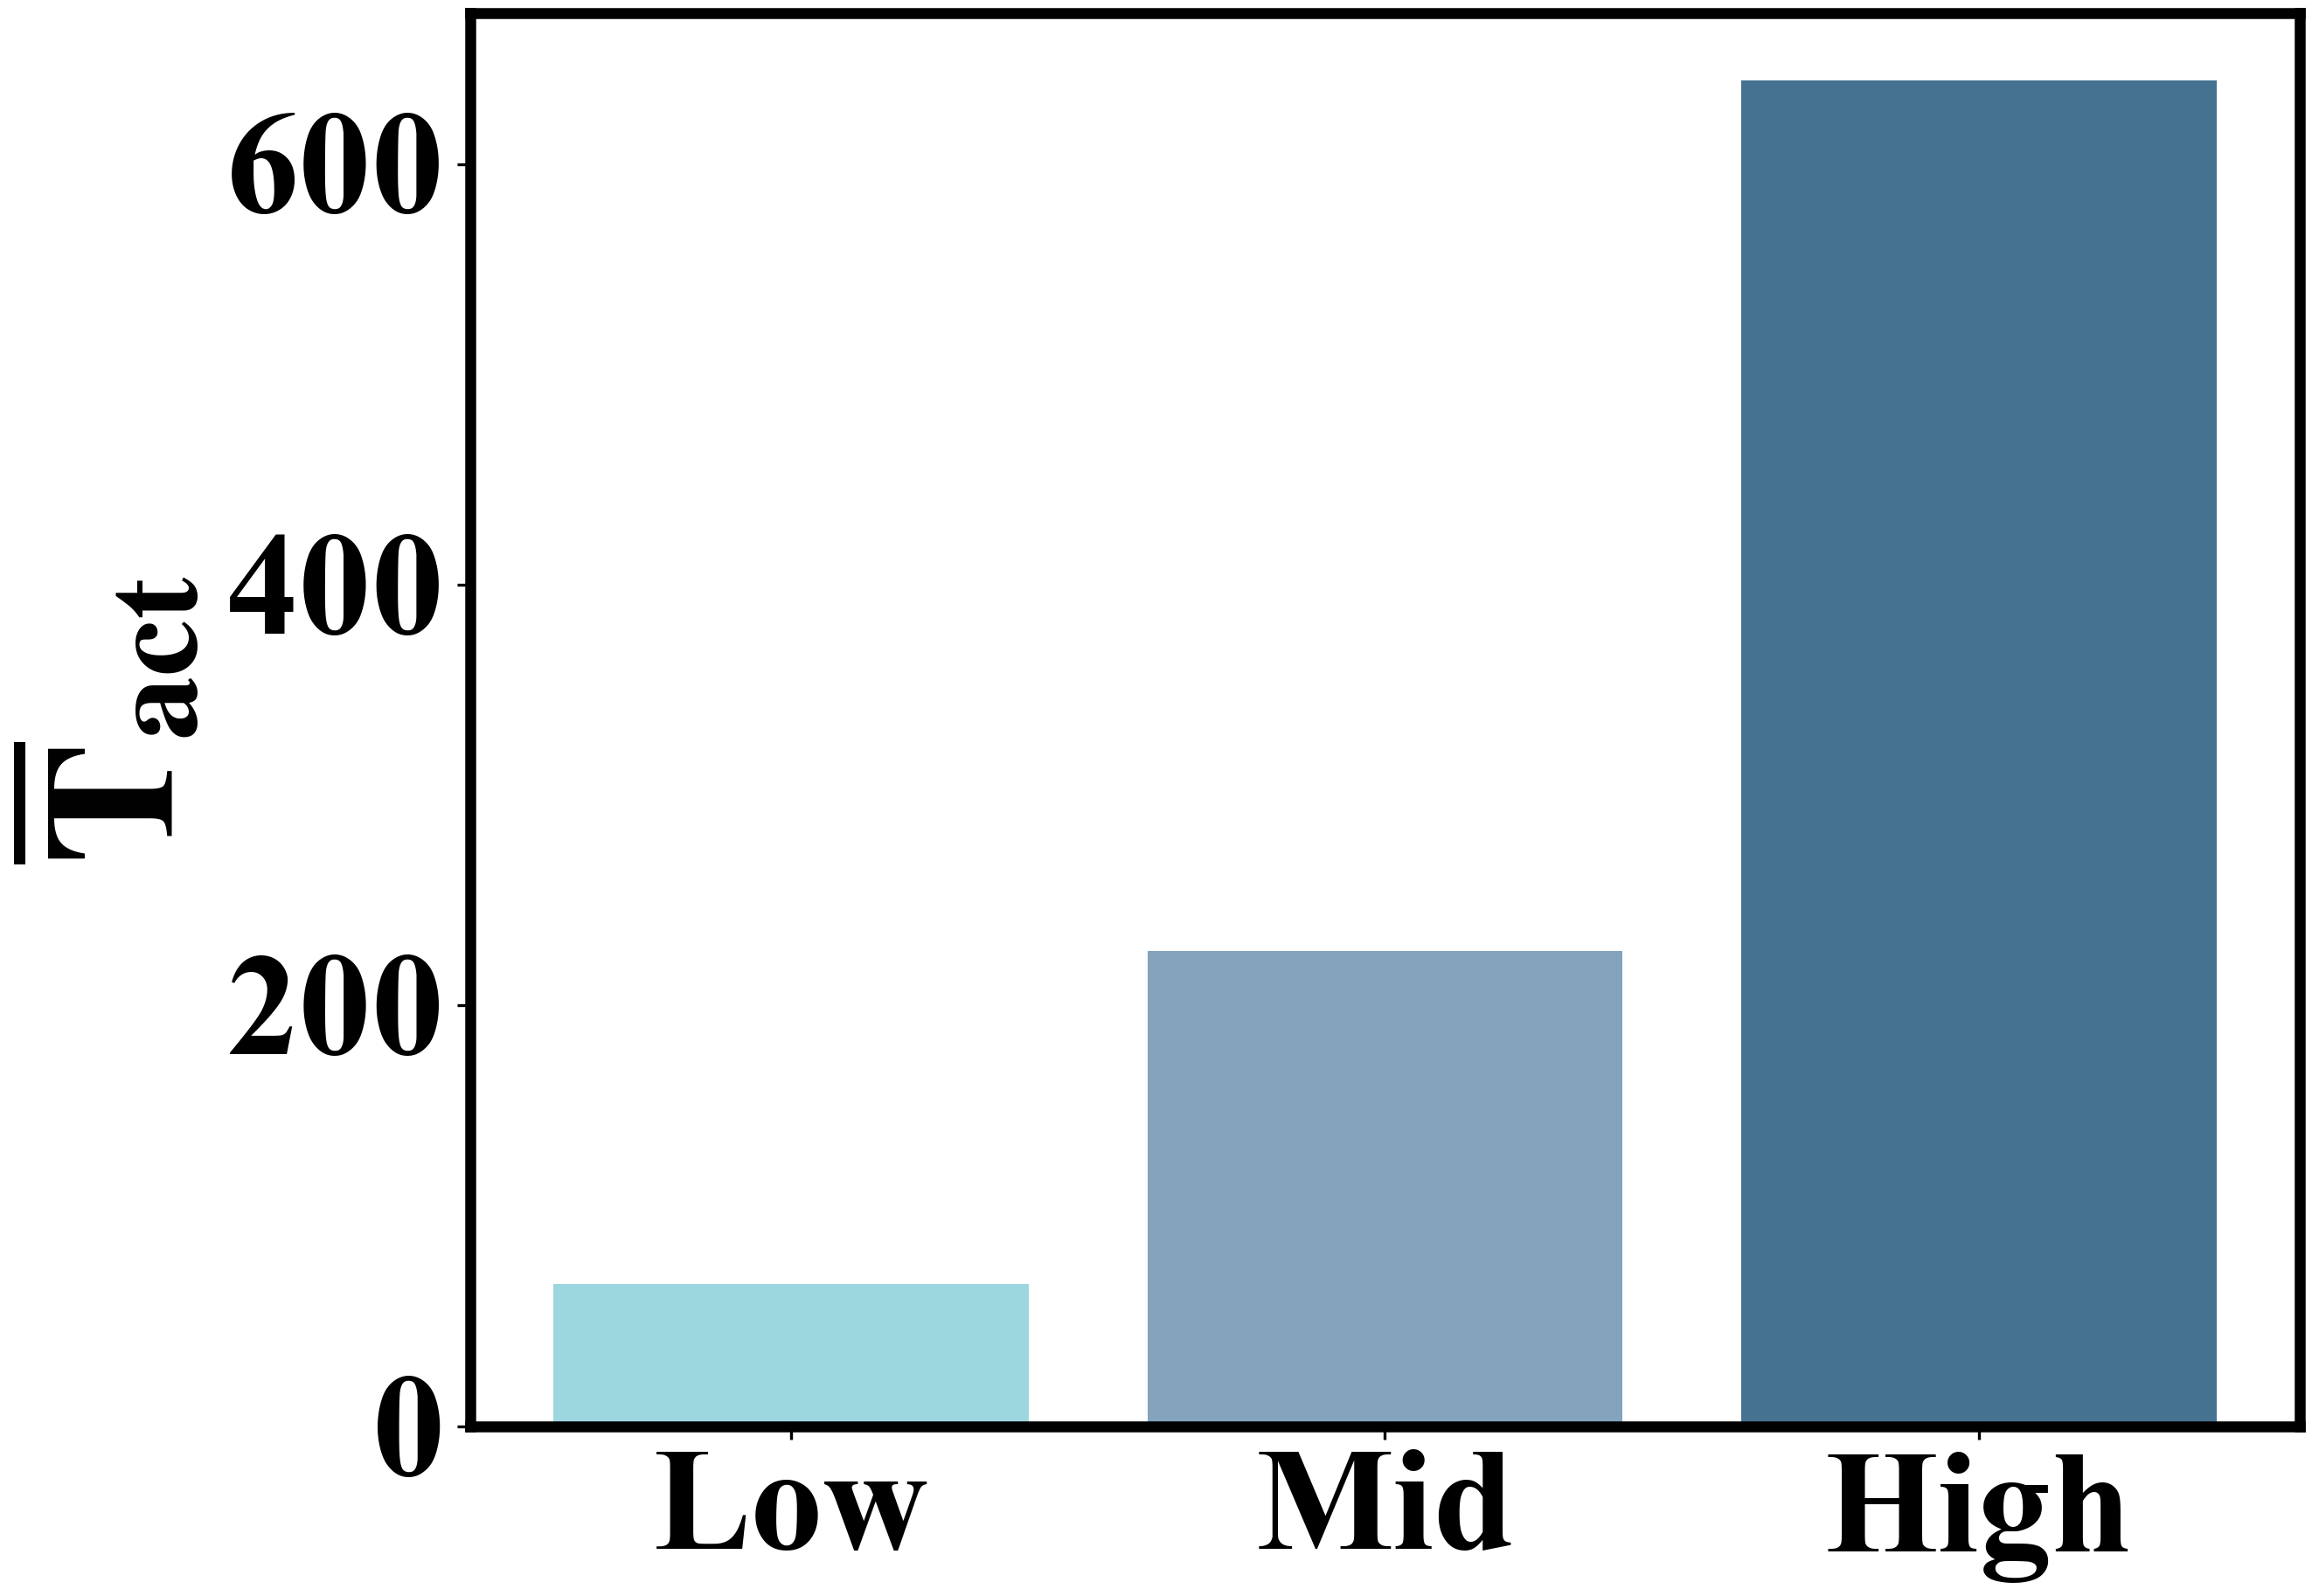}}
	\subcaptionbox{Conformity\label{fig:bar_true_conf}}{
	    \vspace{-6pt}
		\includegraphics[width=0.32\linewidth]{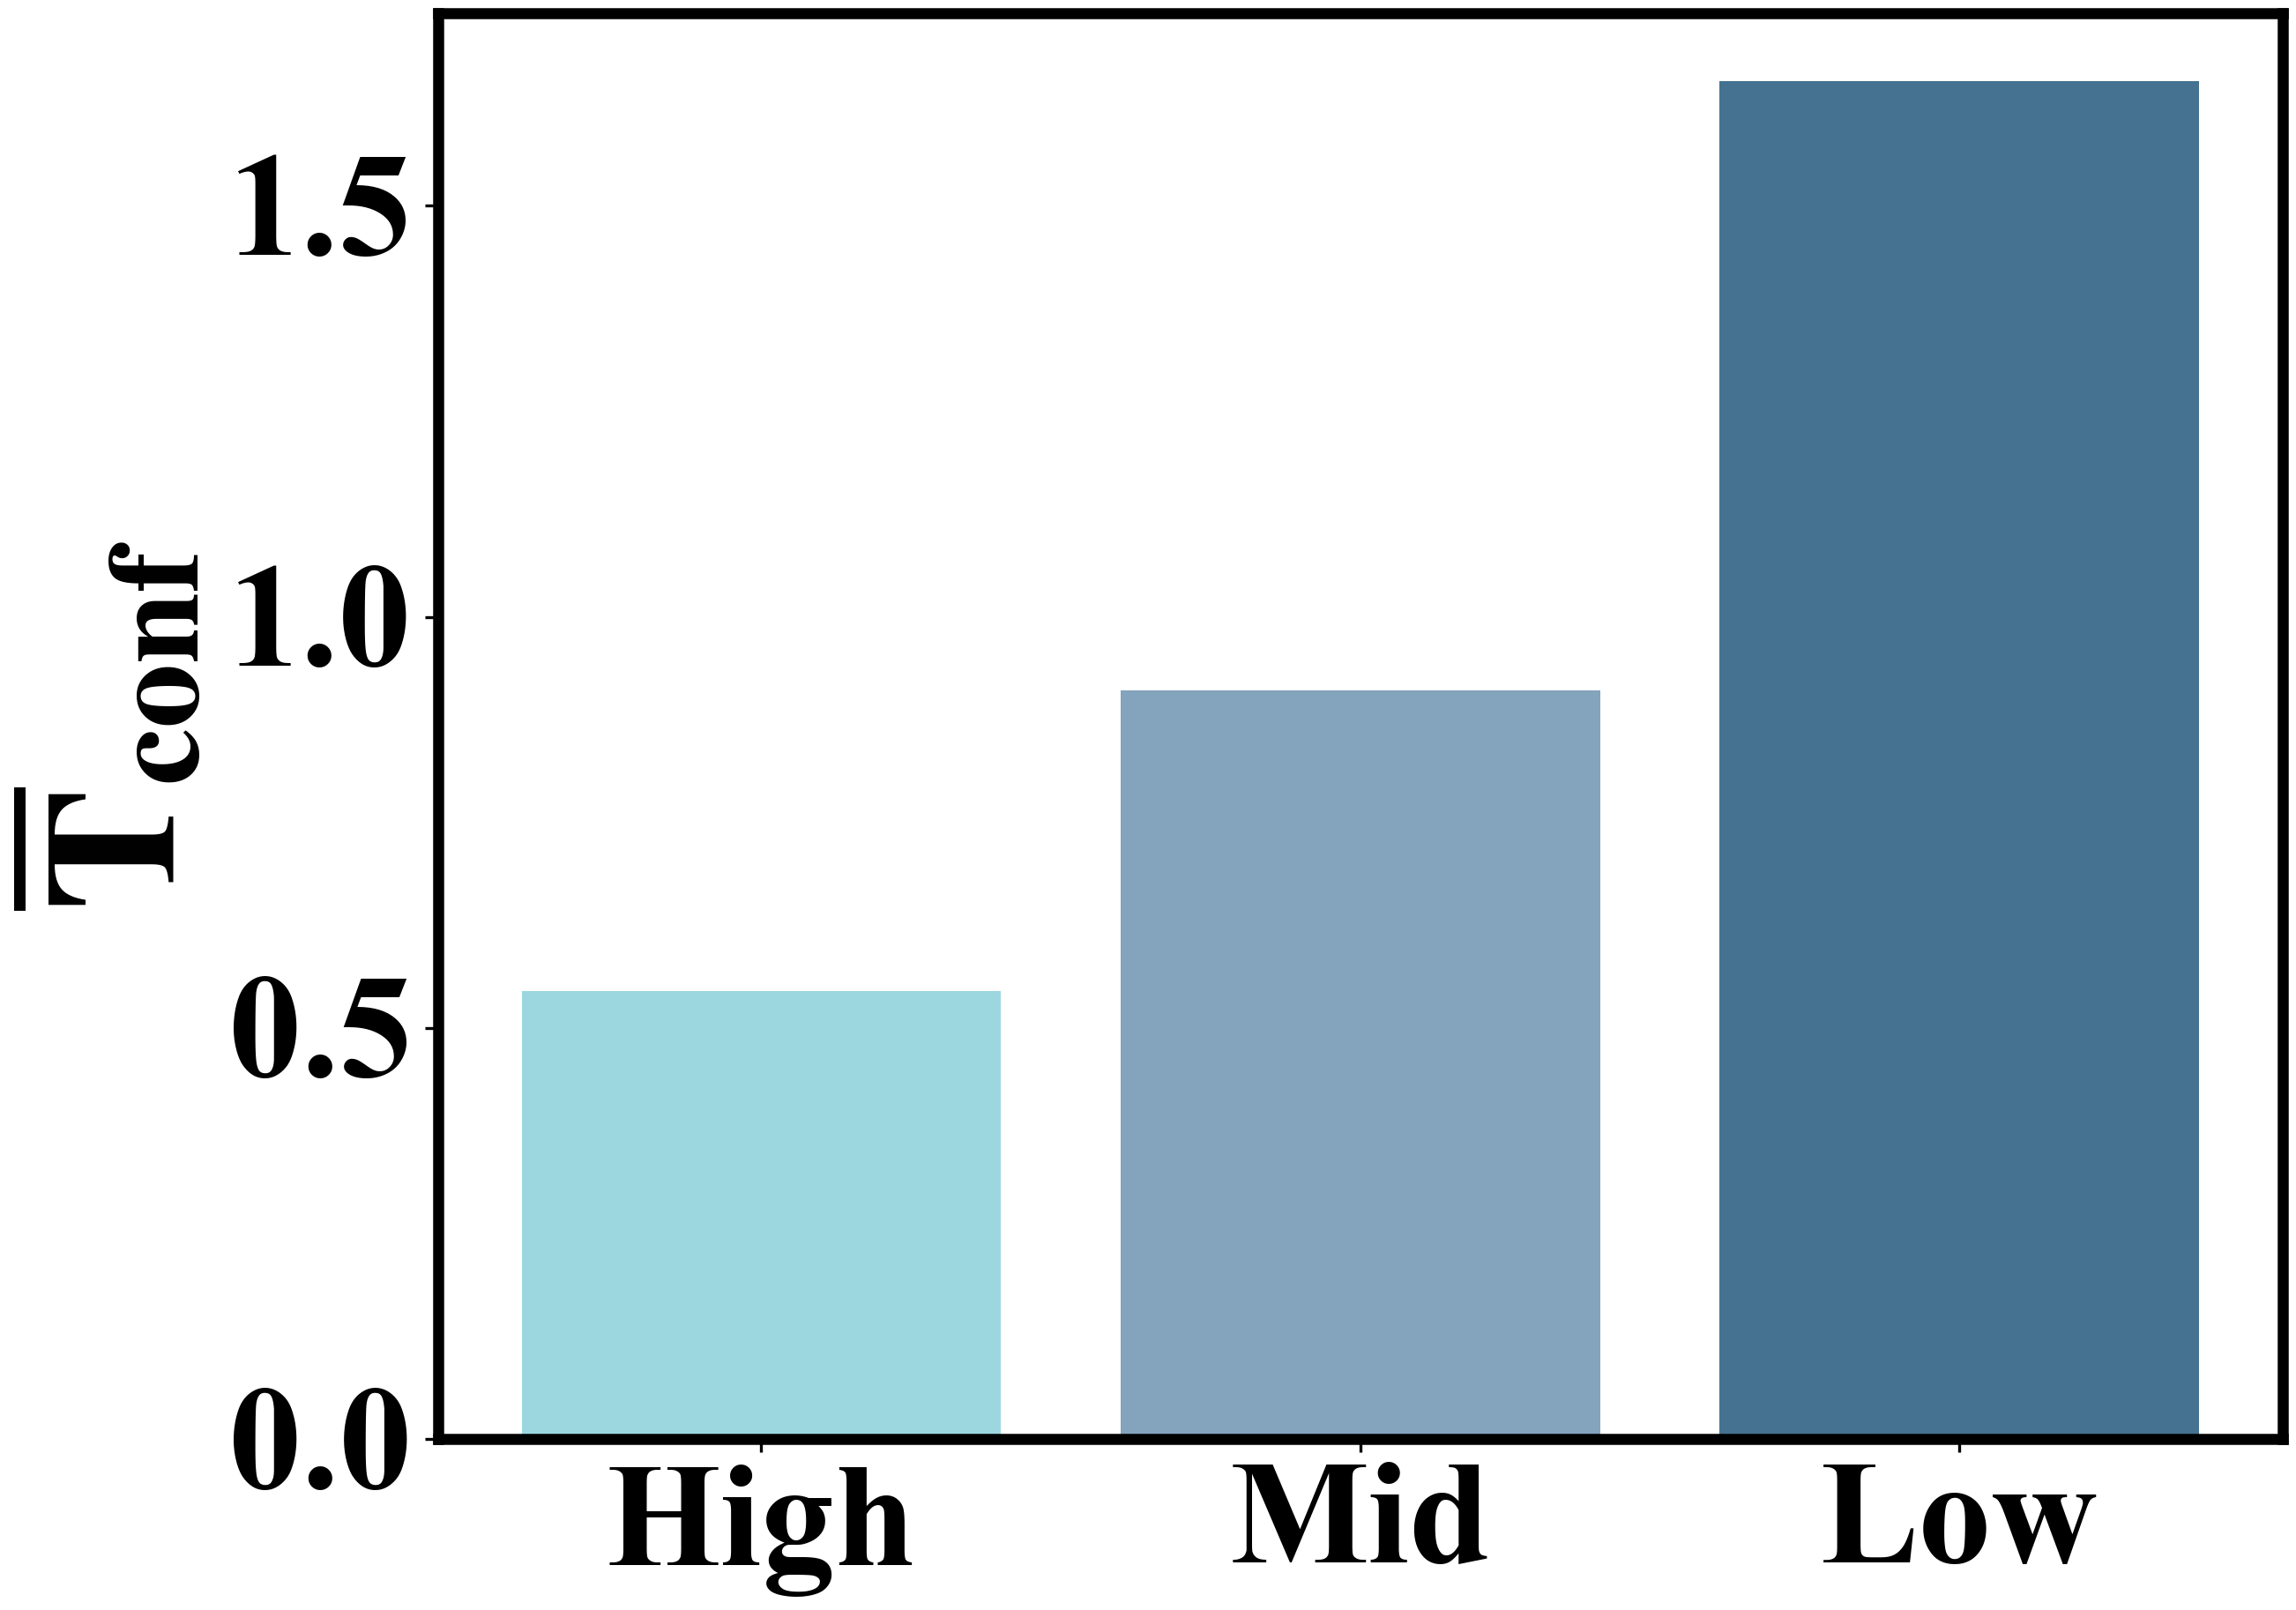}}
	\subcaptionbox{Diversity\label{fig:bar_true_diver}}{
	    \vspace{-6pt}
		\includegraphics[width=0.31\linewidth]{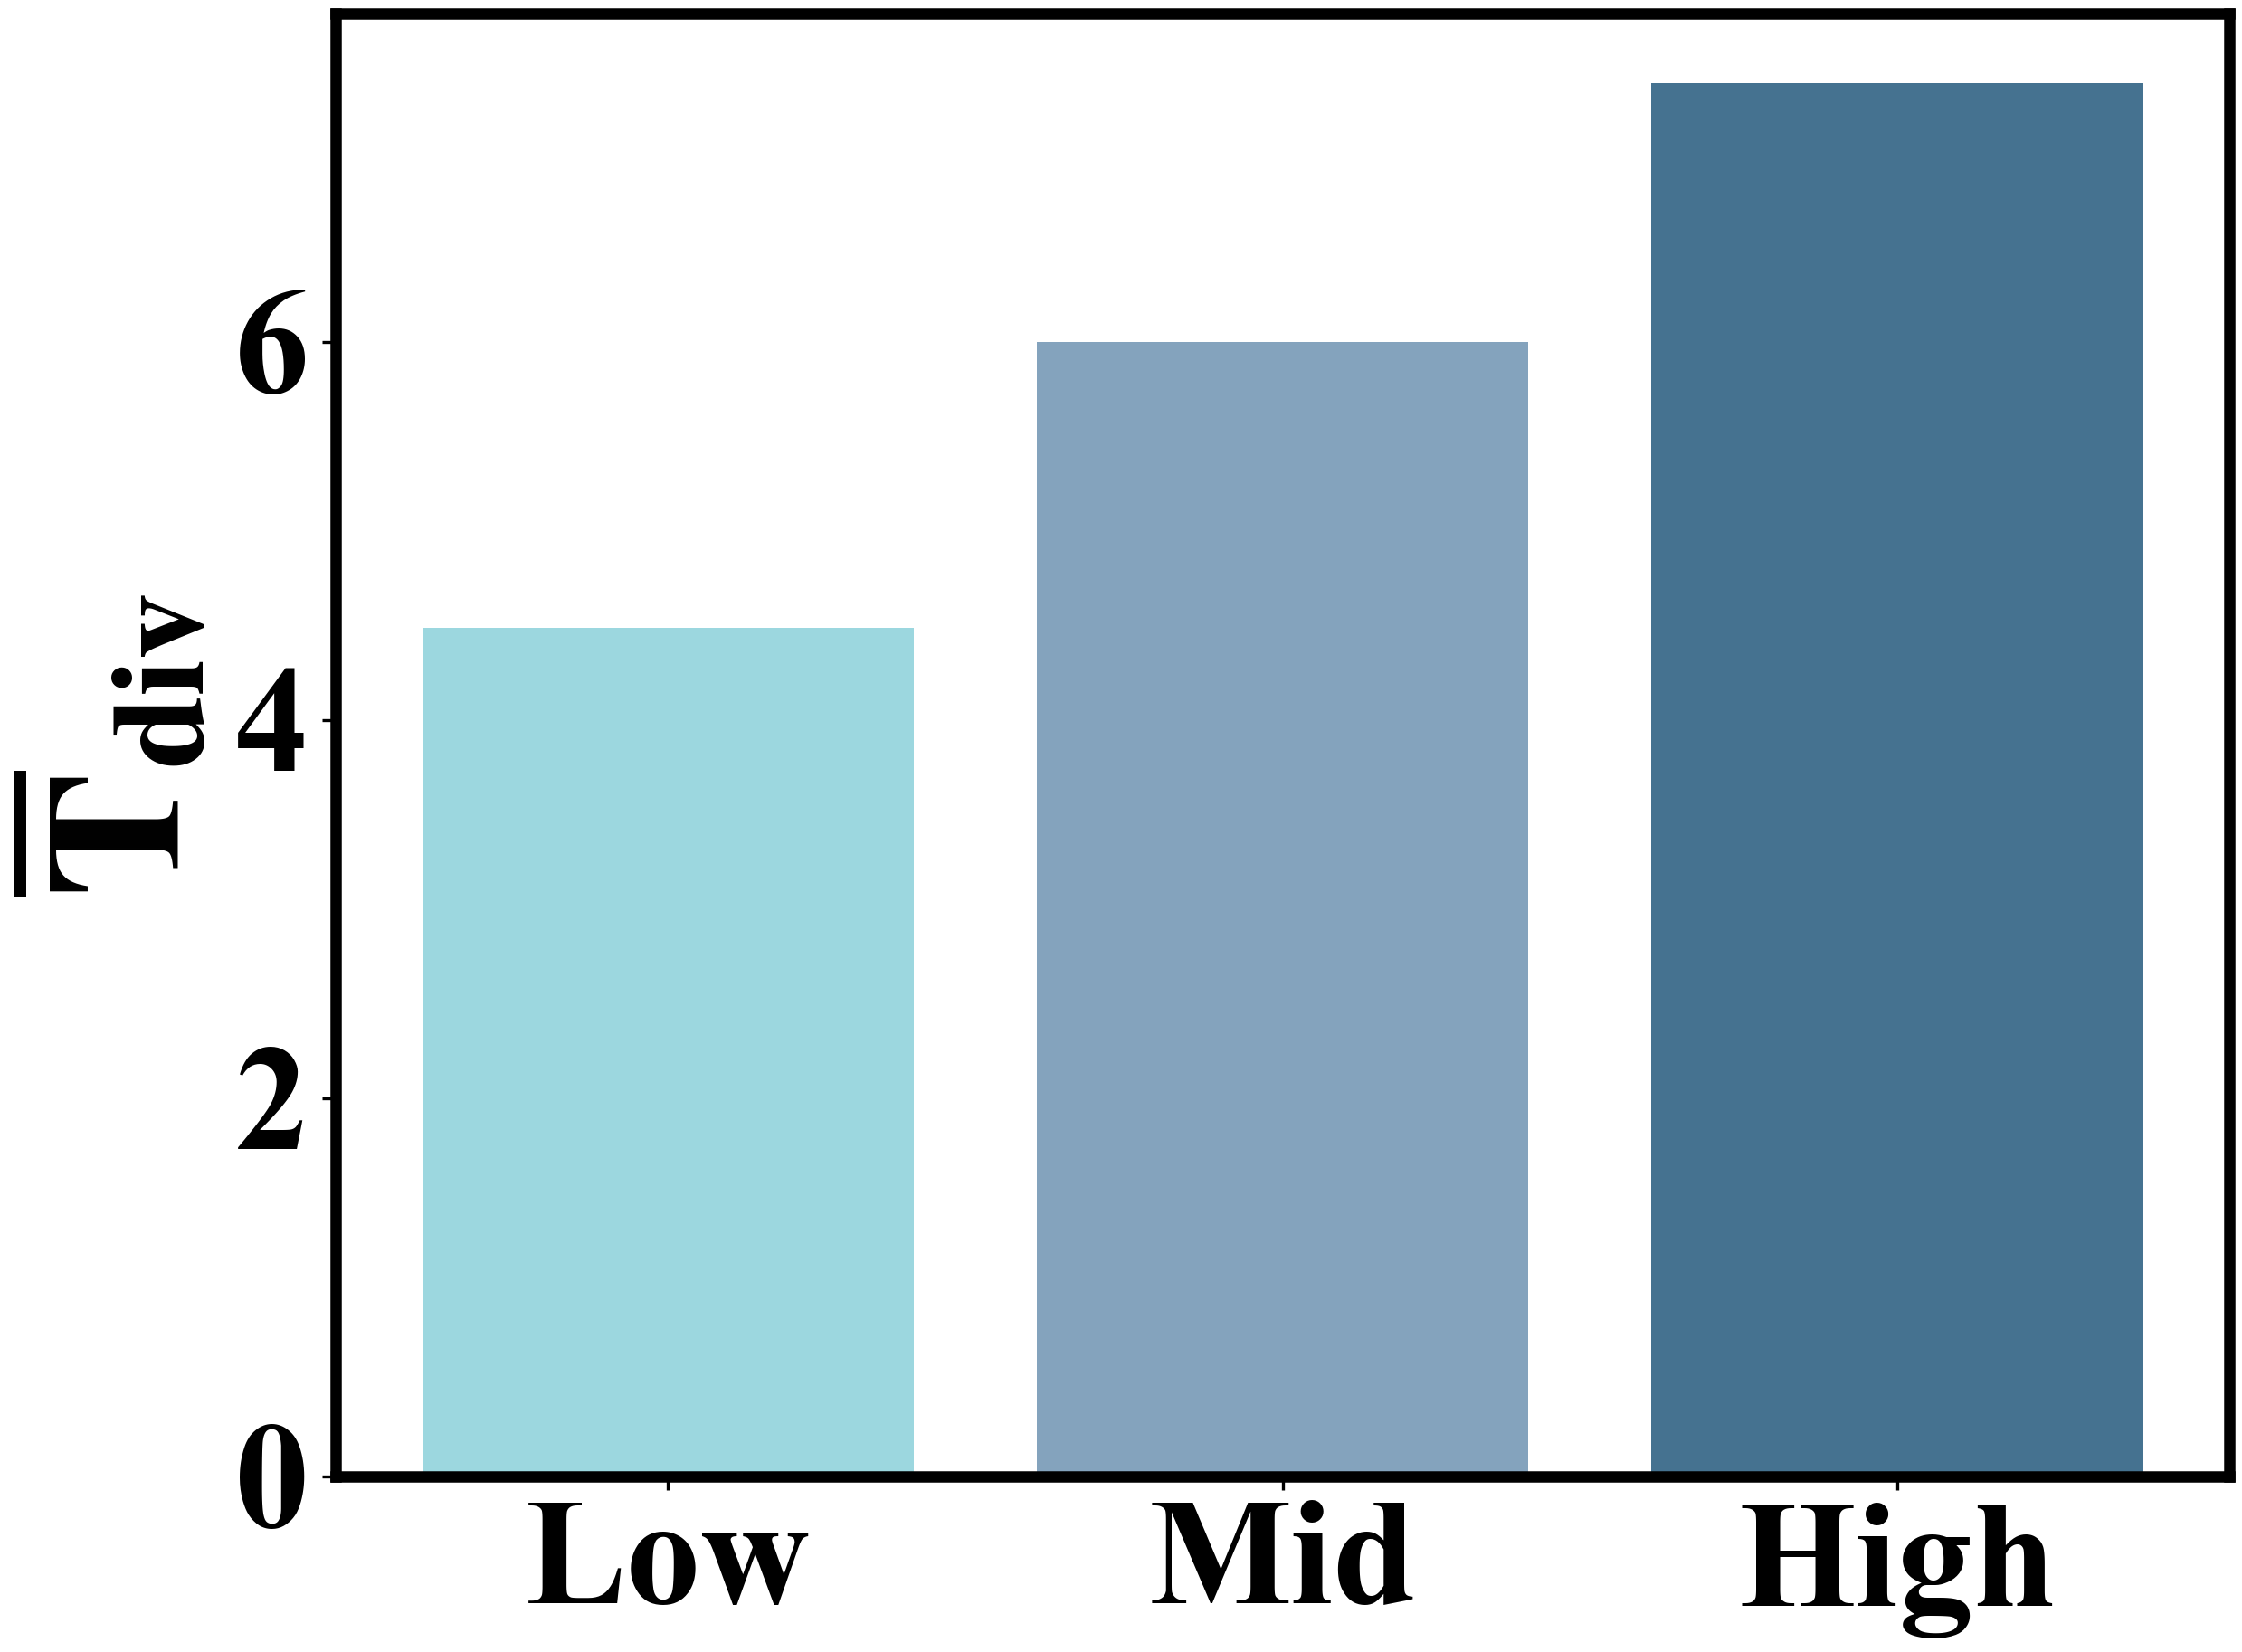}}
	\vspace{-10pt}	
	% \caption{The averaged behavior of human user groups with varying degrees of social traits.}
 	\caption{The averaged social traits of human user within different traits groups.}
	\label{fig:group_true}
	\vspace{-10pt}
\end{figure}
\begin{figure}[t]
	\centering
	\subcaptionbox{w Conformity trait\label{fig:conf_hist}}{
	    \vspace{-5pt}
		\includegraphics[width=0.47\linewidth]{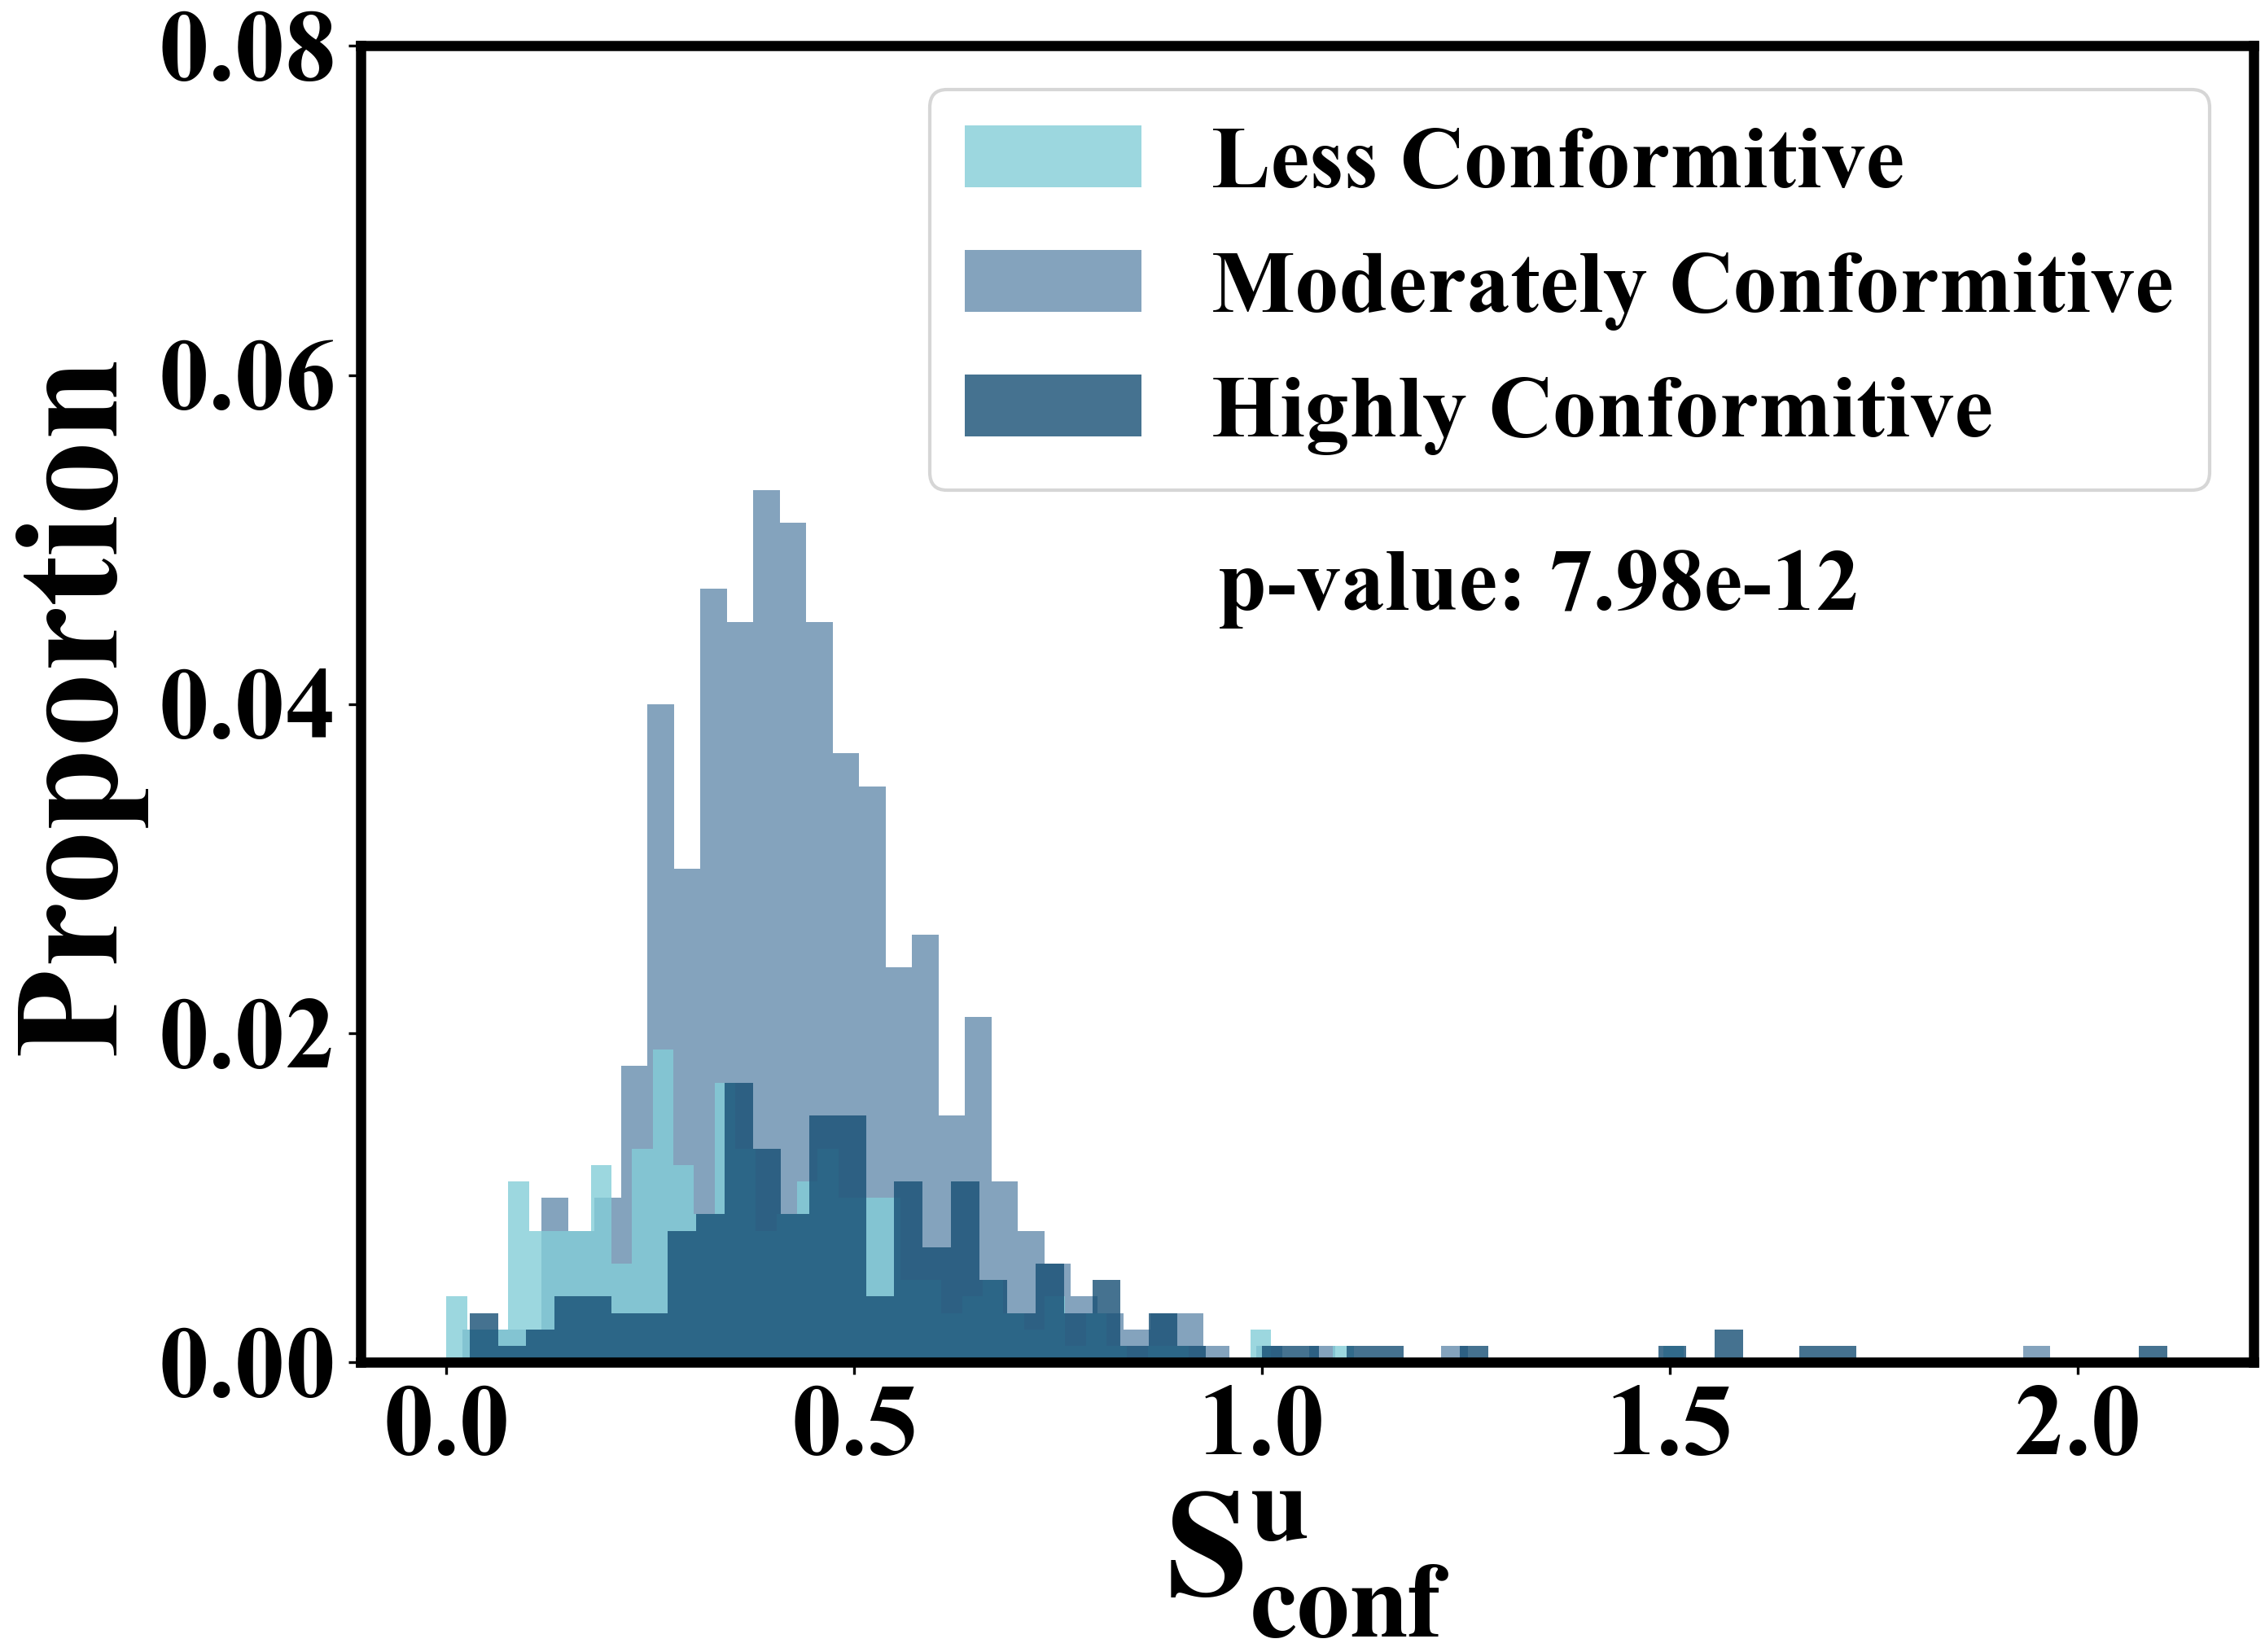}}
	\subcaptionbox{w/o Conformity trait\label{fig:conf_hist_abl}}{
	    \vspace{-5pt}
		\includegraphics[width=0.47\linewidth]{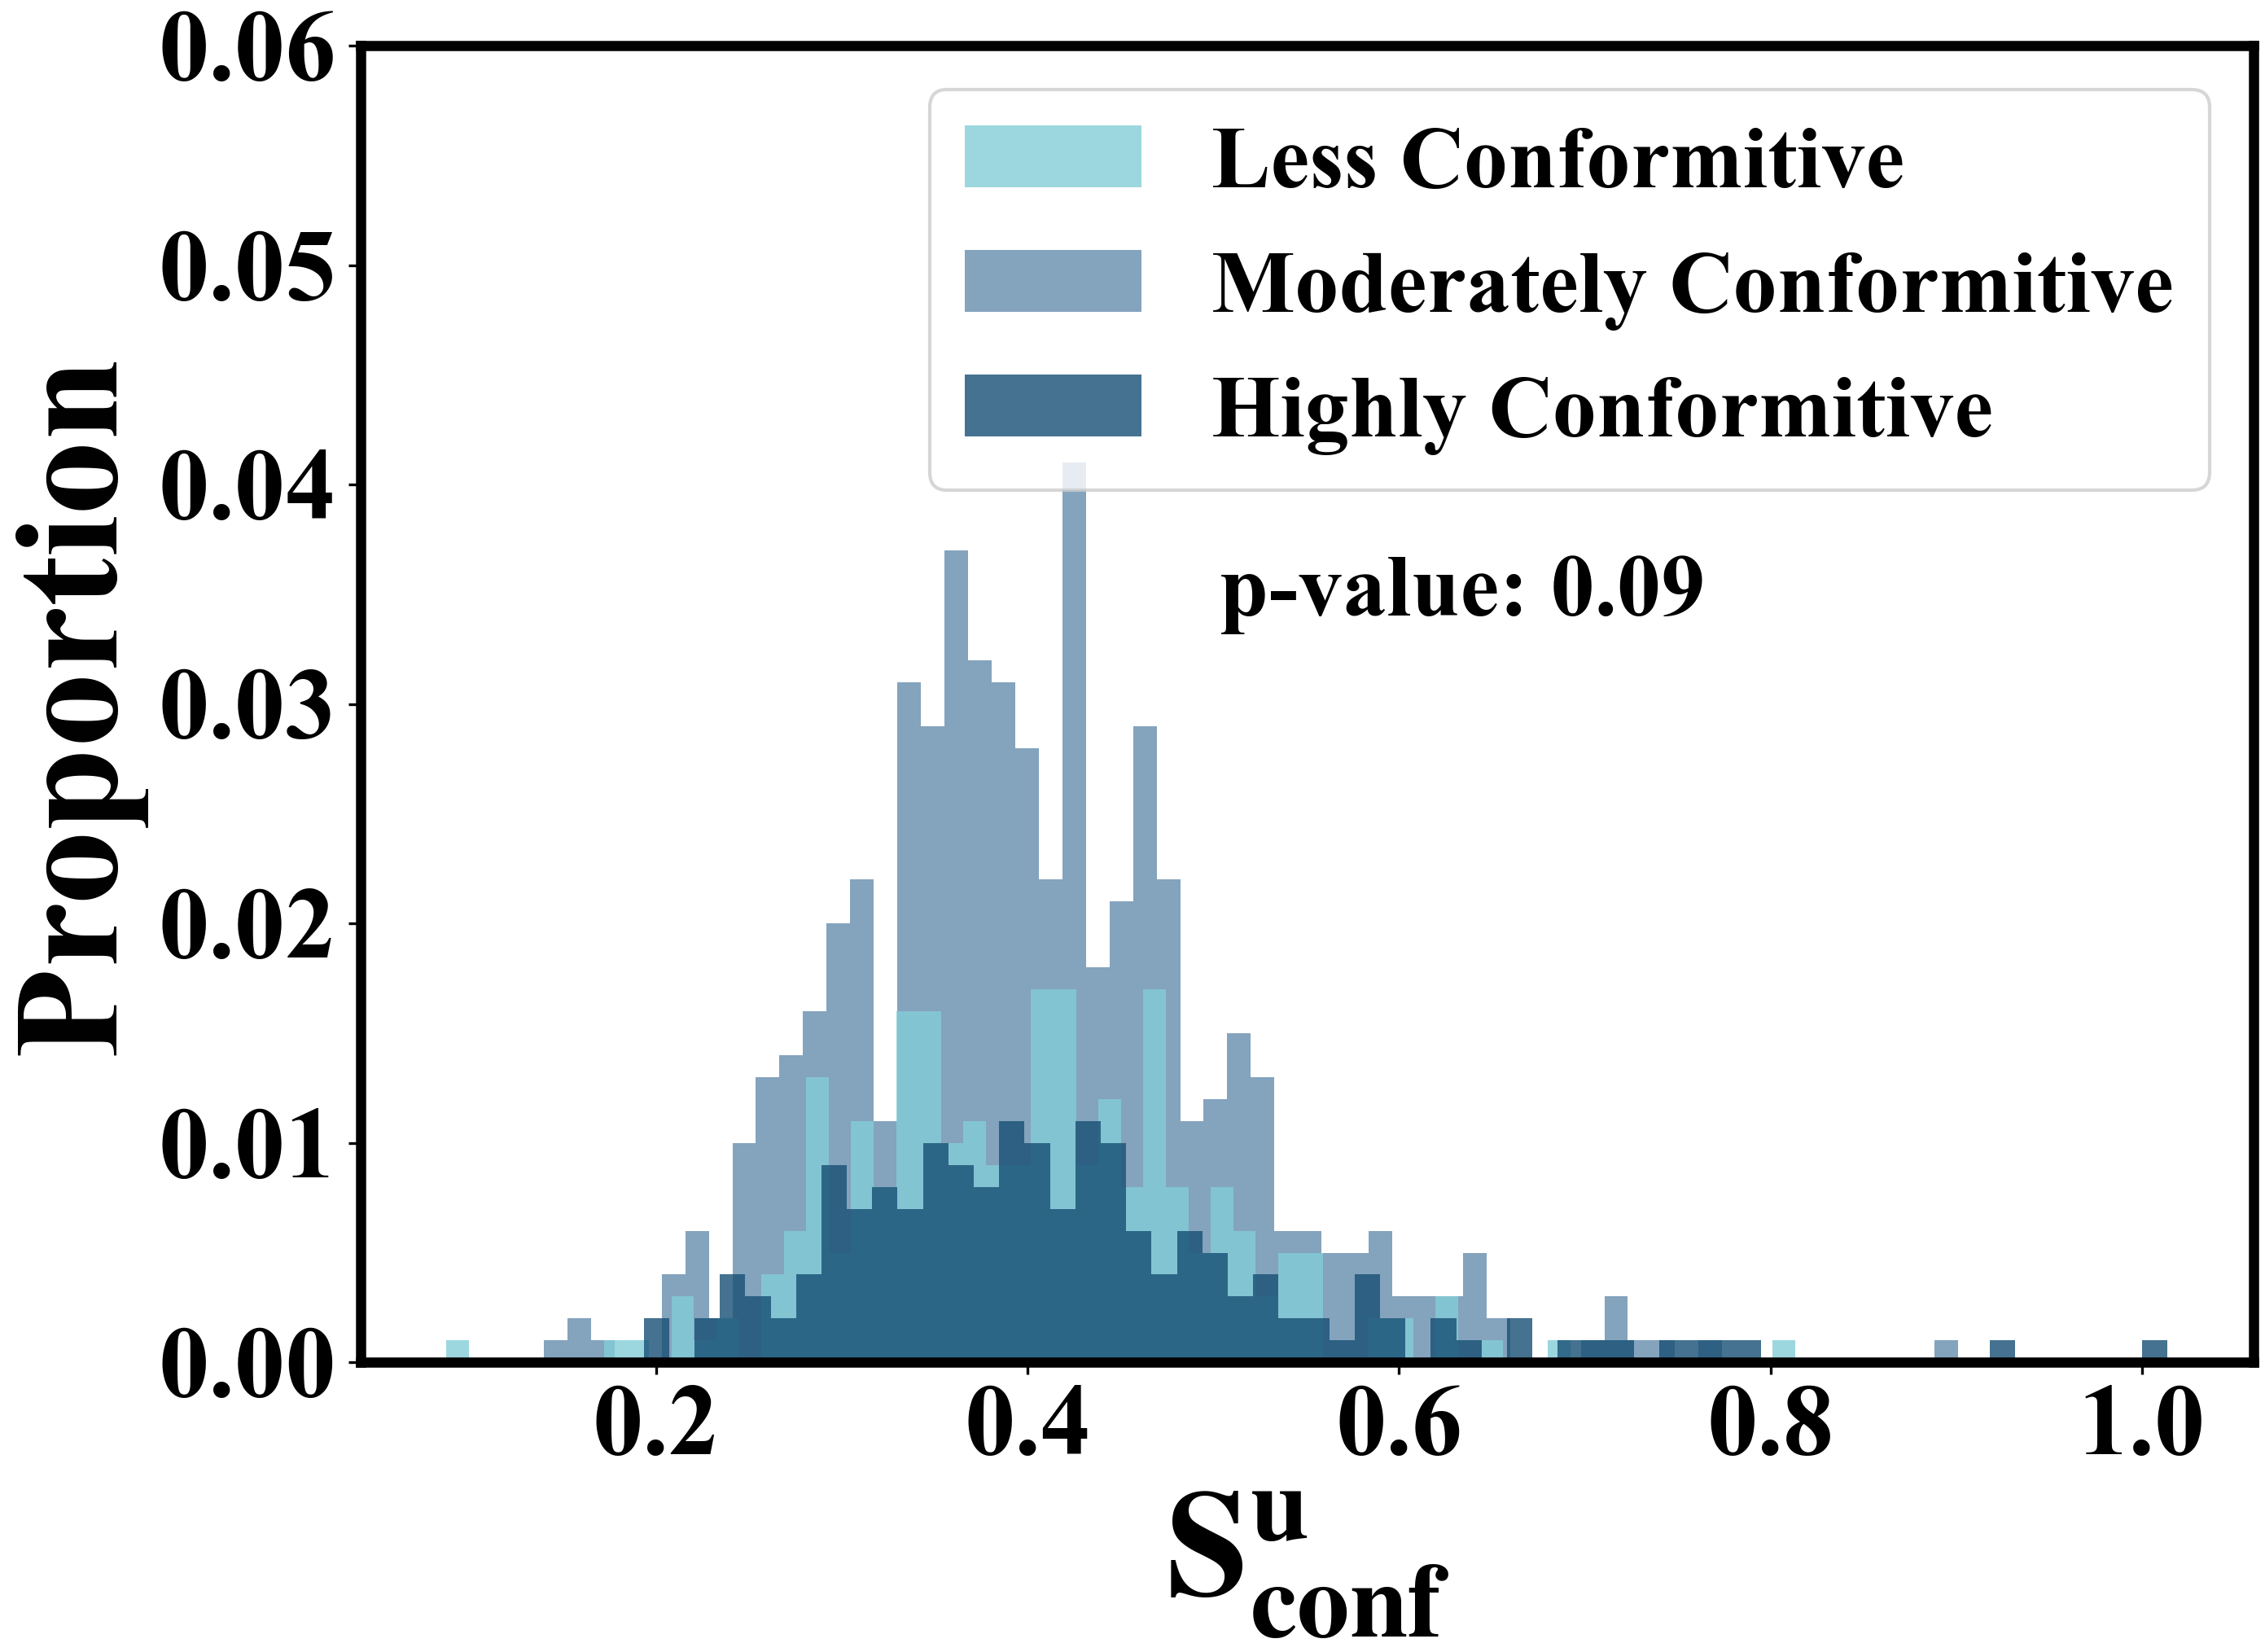}}
	\vspace{-10pt}	
	\caption{An ablation study illustrating the distribution of \slh{conformity scores} among agents with varying levels of user conformity.}
	\label{fig:hist_conf}
	\vspace{-10pt}
\end{figure}

\begin{figure}[t]
	\centering
	\subcaptionbox{w Diversity trait\label{fig:diver_hist}}{
	    \vspace{-5pt}
		\includegraphics[width=0.47\linewidth]{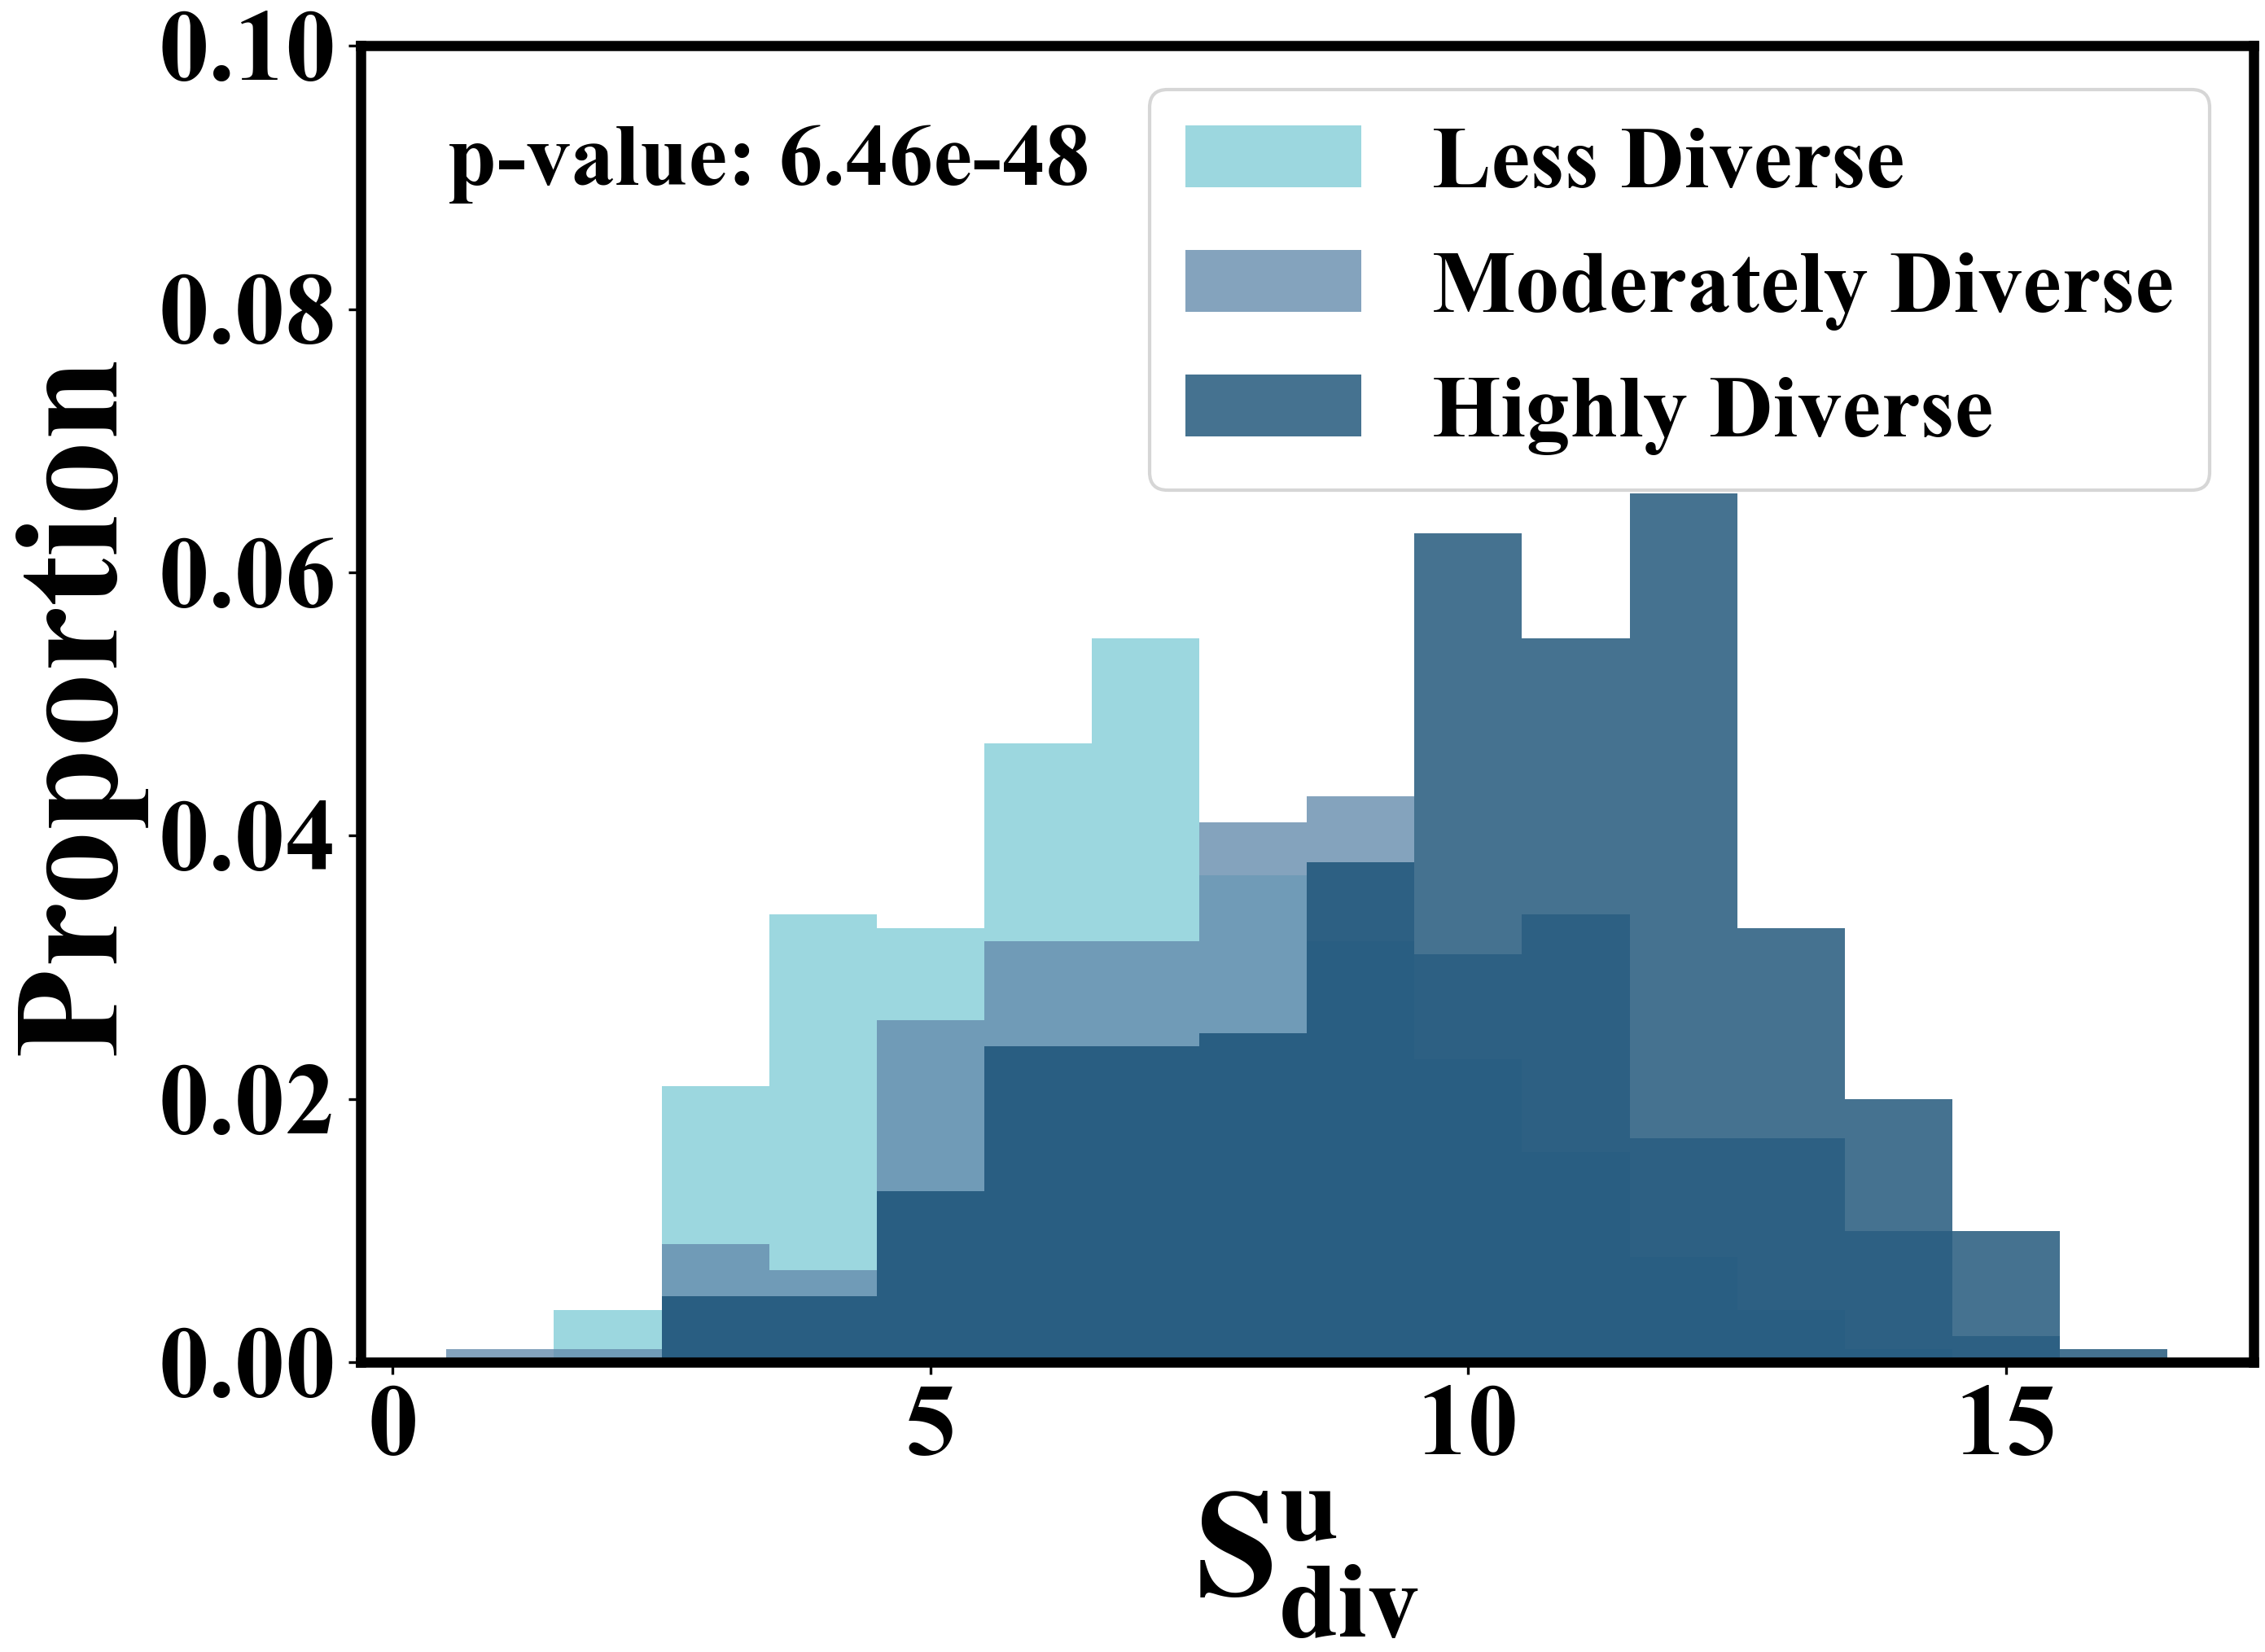}}
	\subcaptionbox{w/o Diversity trait\label{fig:diver_hist_abl}}{
	    \vspace{-5pt}
		\includegraphics[width=0.47\linewidth]{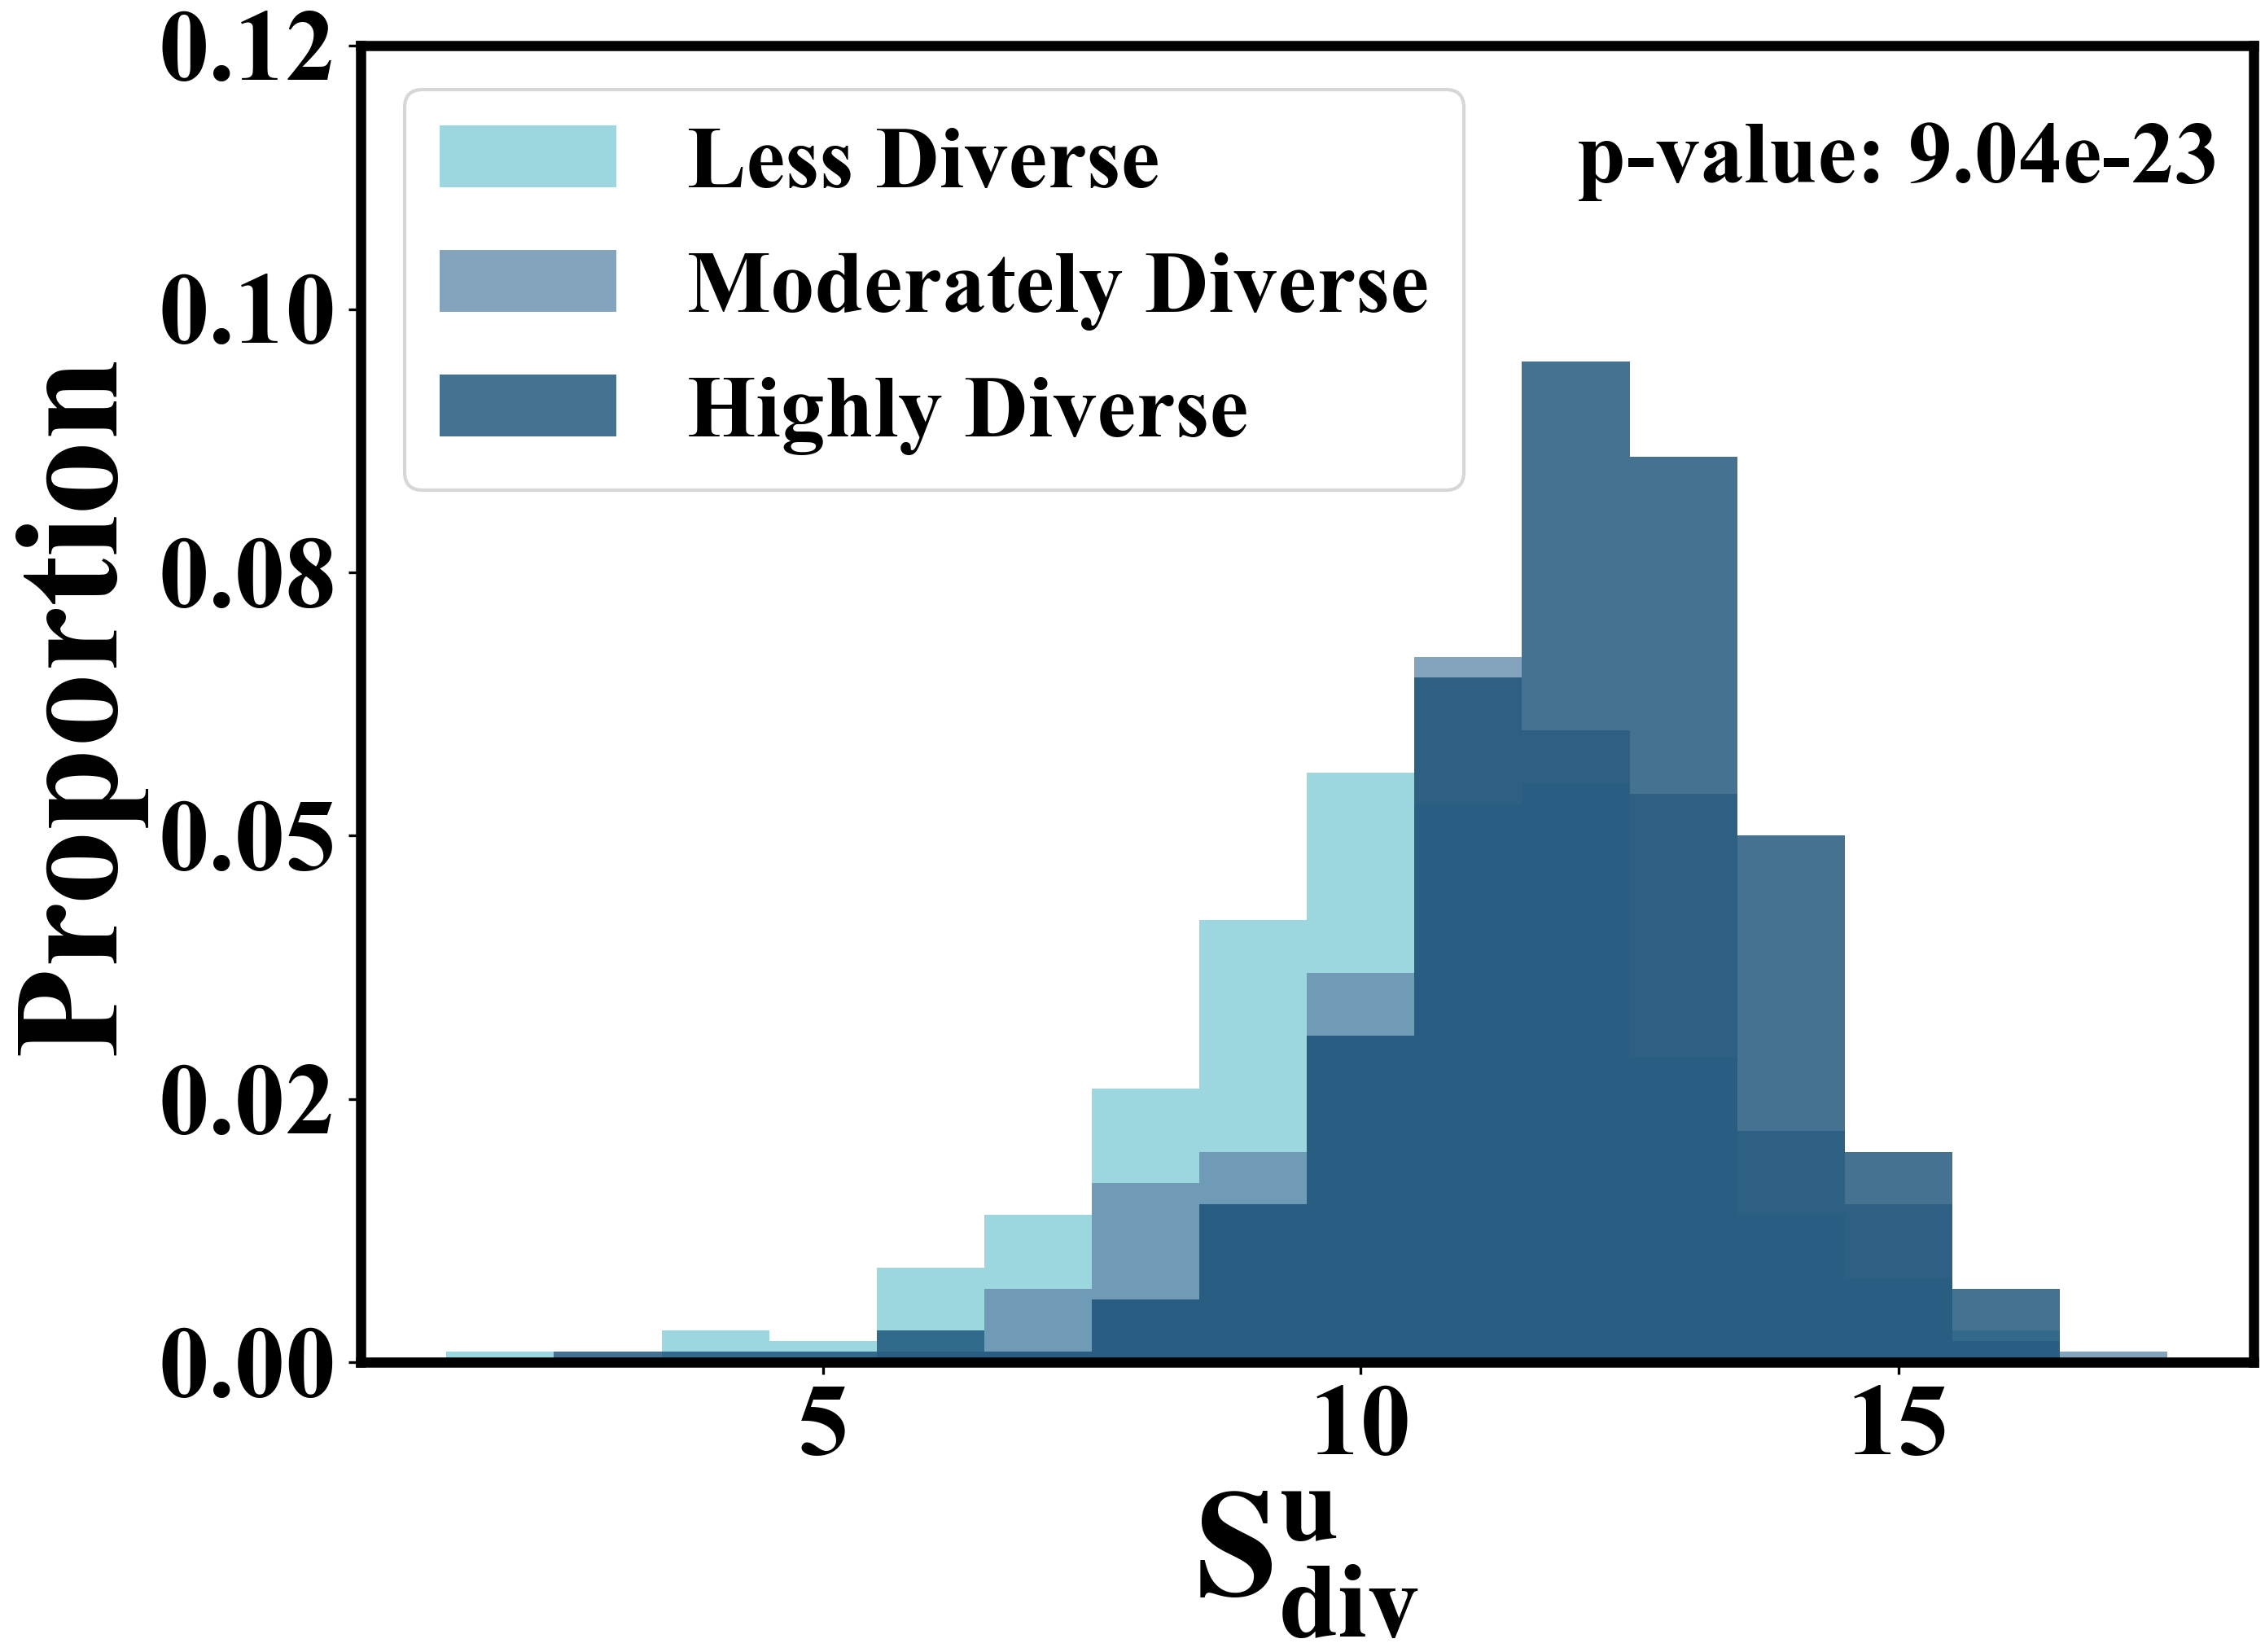}}
	\vspace{-10pt}	
	\caption{An ablation study illustrating the distribution of \slh{diversity score} among agents with varying levels of user diversity.}
	\label{fig:hist_diver}
	\vspace{-10pt}
\end{figure}

\begin{figure}[t]
	\centering
	\subcaptionbox{Ground-truth activity\label{fig:true_act_rolling}}{
	    \vspace{-6pt}
		\includegraphics[width=0.48\linewidth]{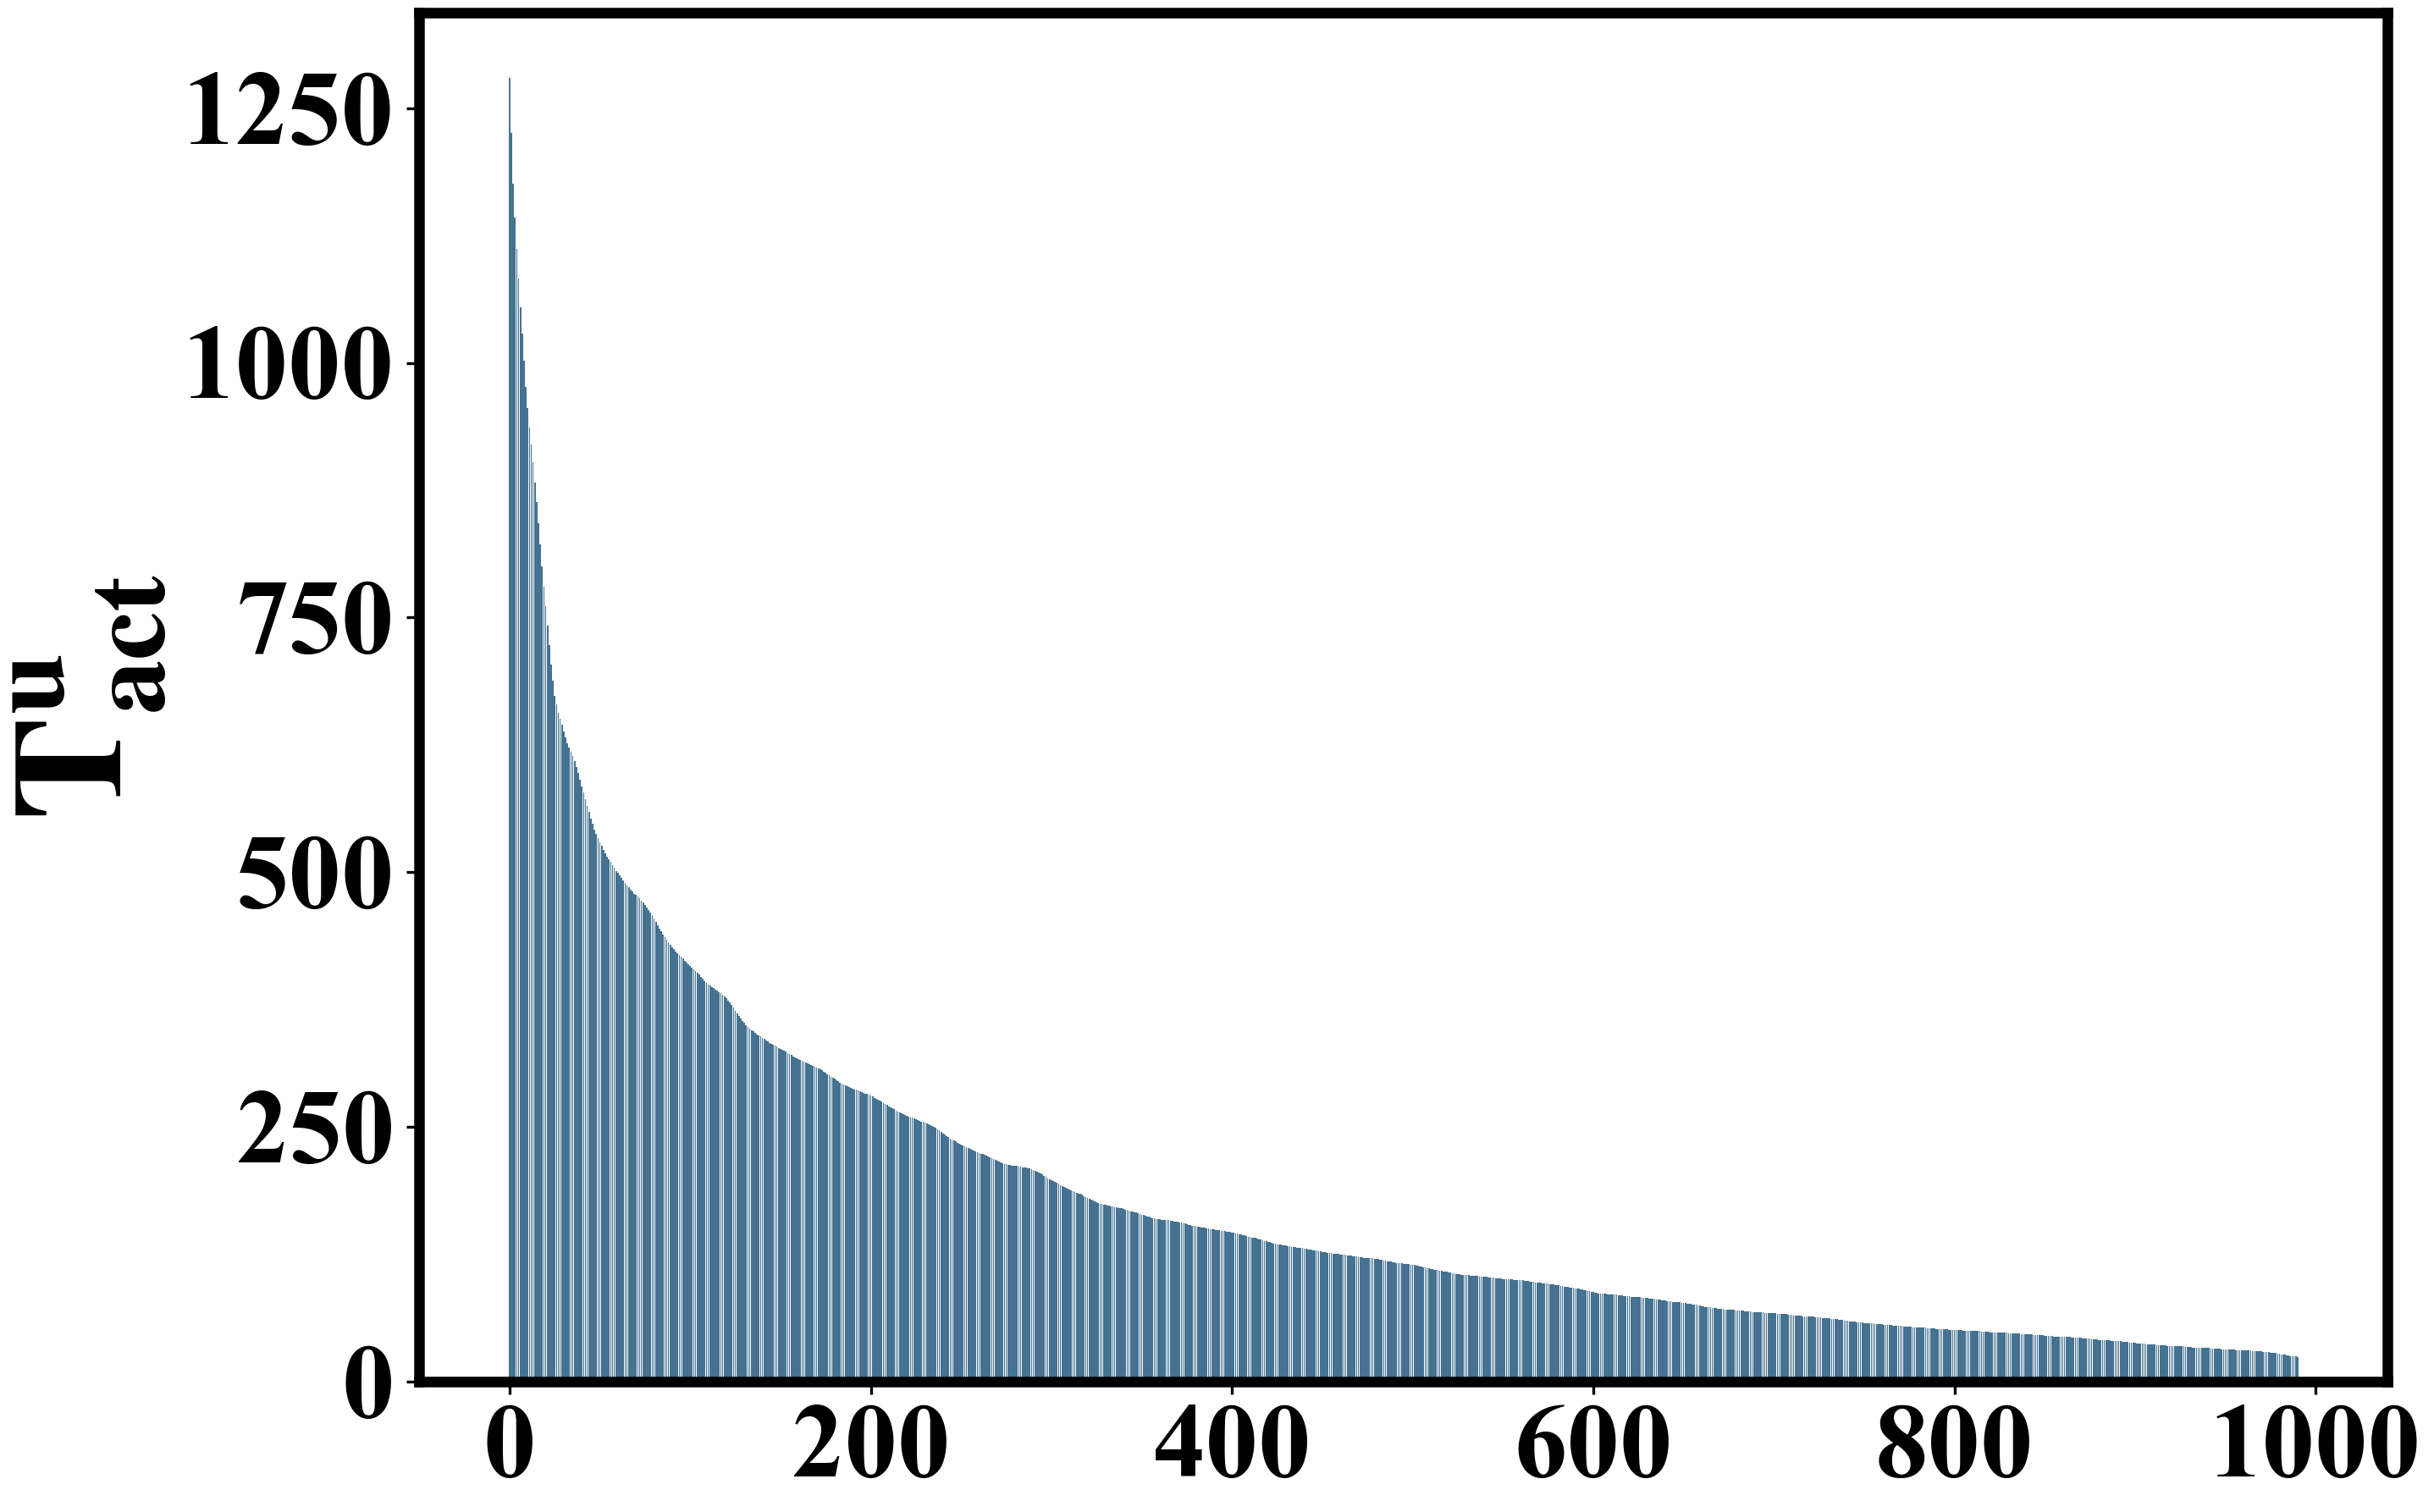}}
	\subcaptionbox{Simulated activity\label{fig:sim_act_rolling}}{
	    \vspace{-6pt}
		\includegraphics[width=0.46\linewidth]{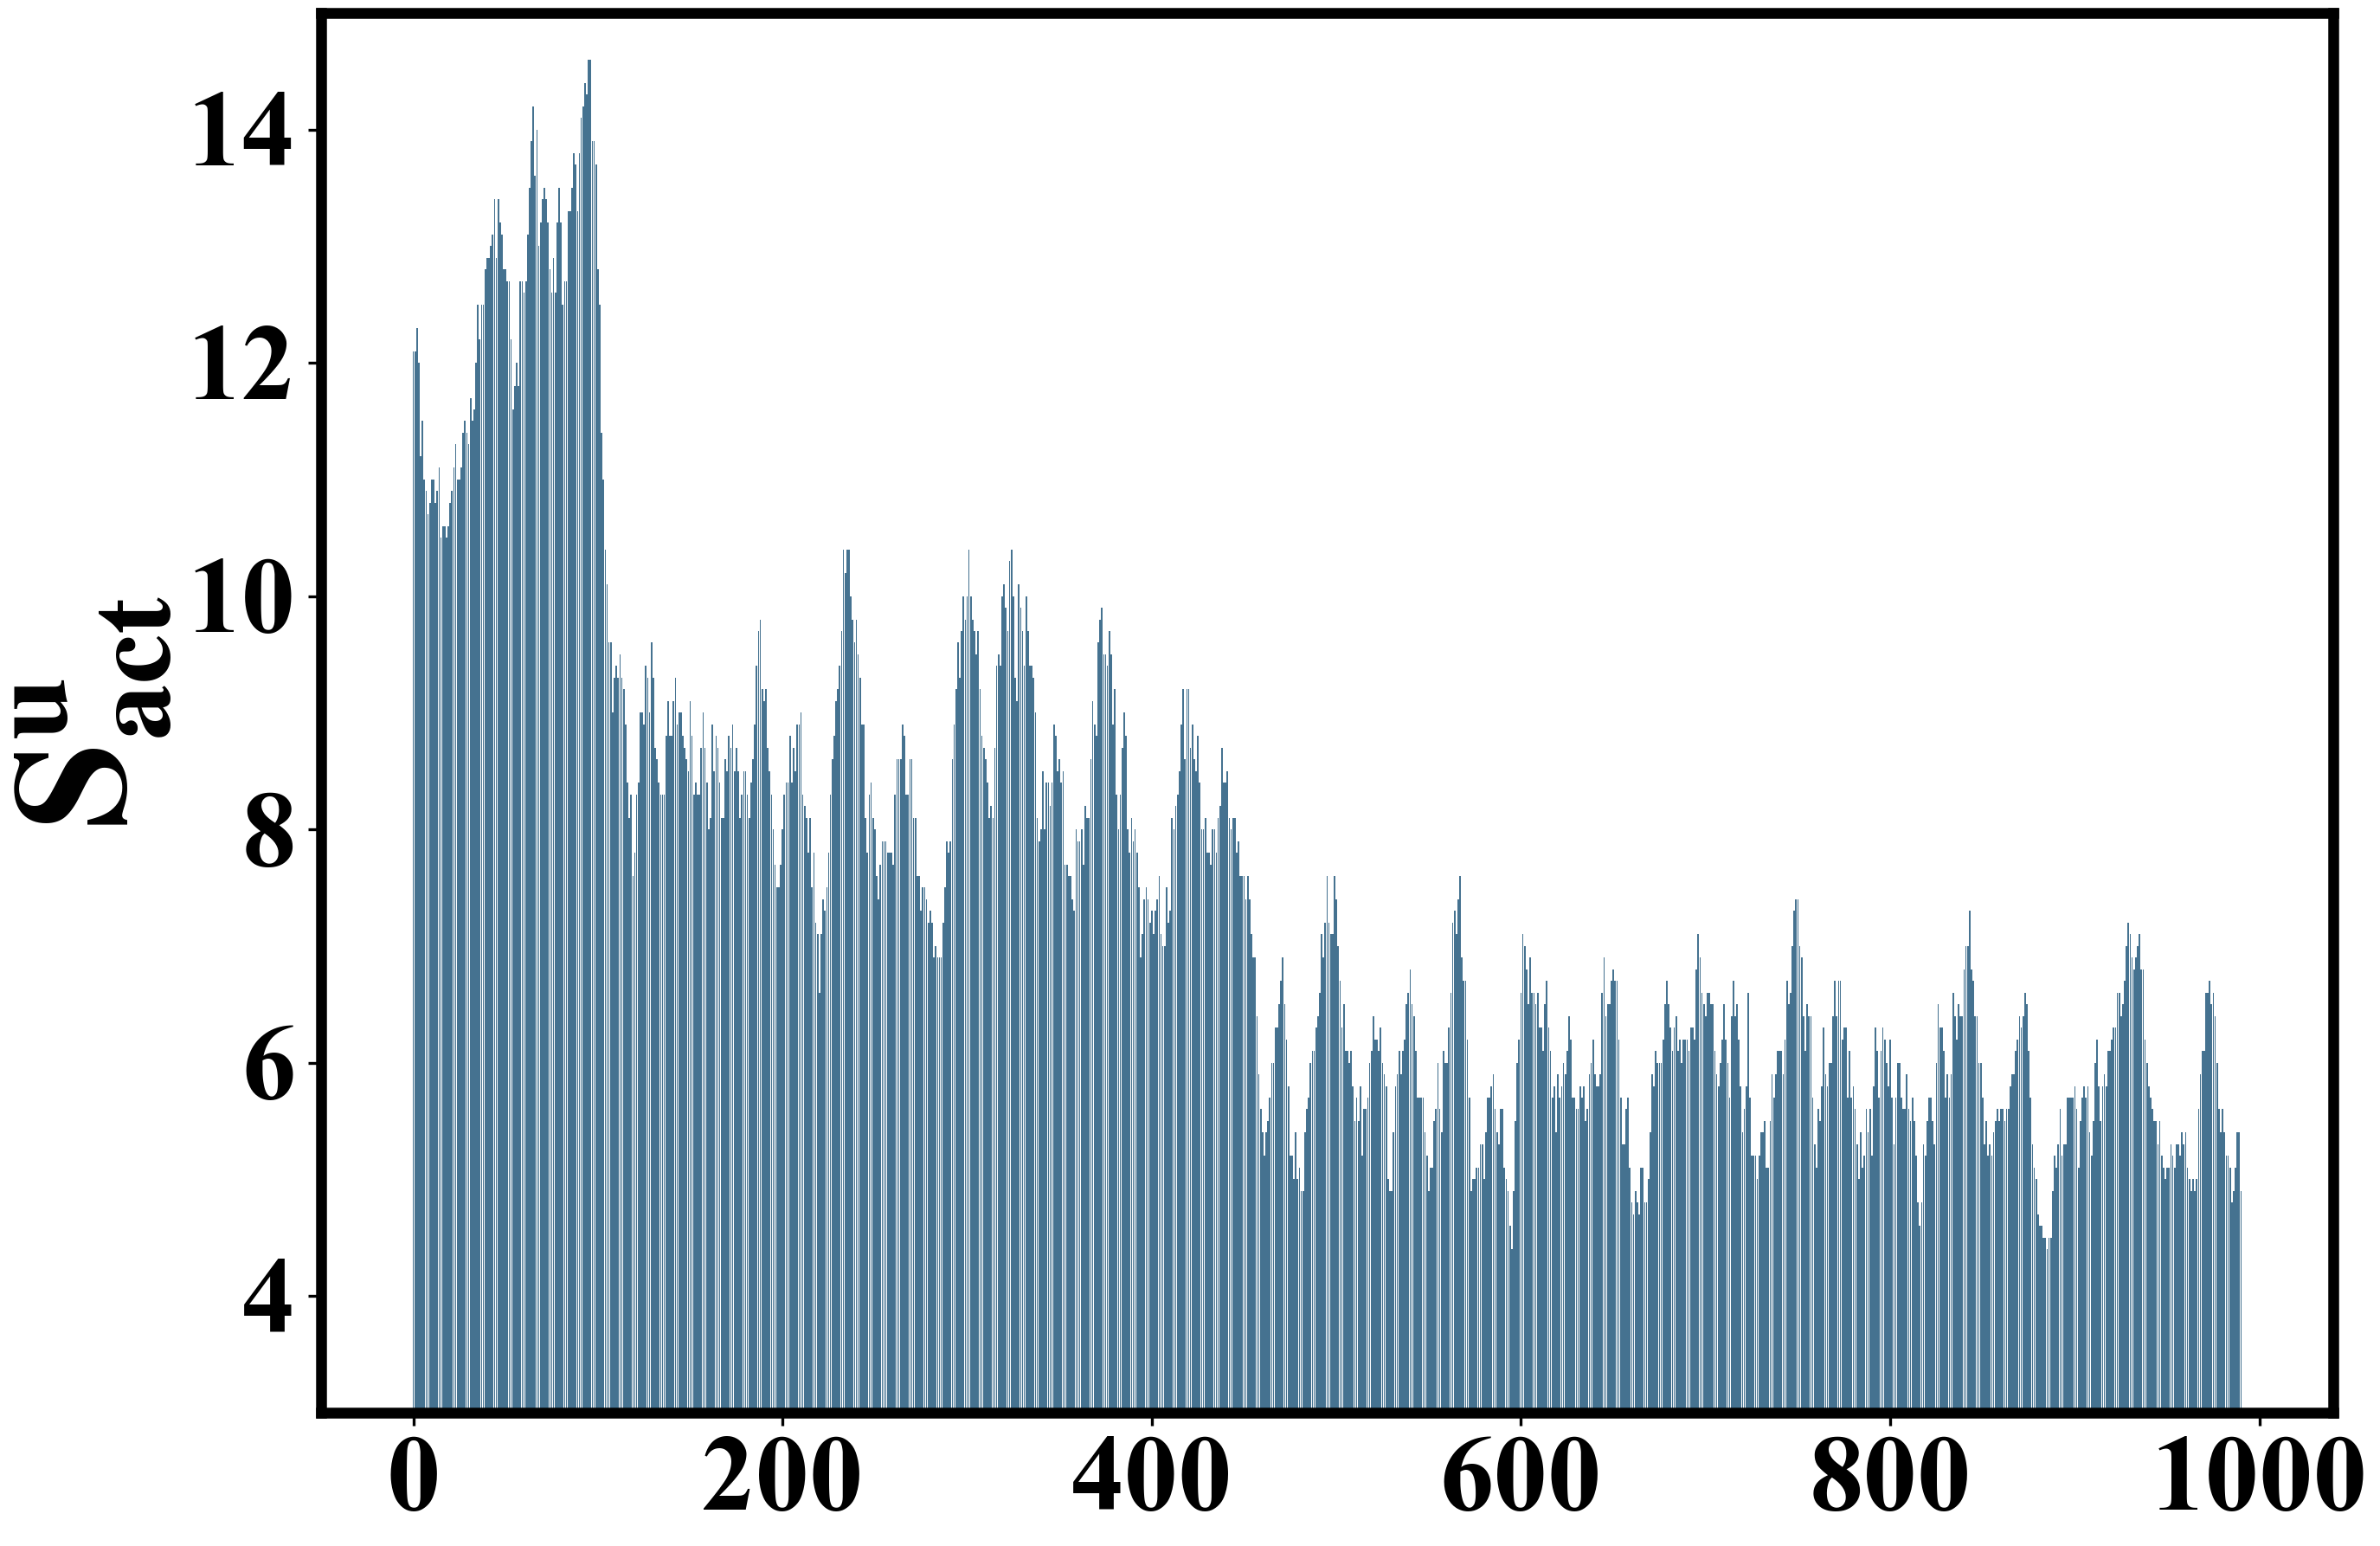}}
	\vspace{-10pt}	
	\caption{A comparison between the distributions of ground-truth activity and activity scores simulated by agents.}
	\label{fig:rolling_act}
	\vspace{-10pt}
\end{figure}

\begin{figure}[t]
	\centering
	\subcaptionbox{Ground-truth conformity\label{fig:true_conf_rolling}}{
	    \vspace{-6pt}
		\includegraphics[width=0.46\linewidth]{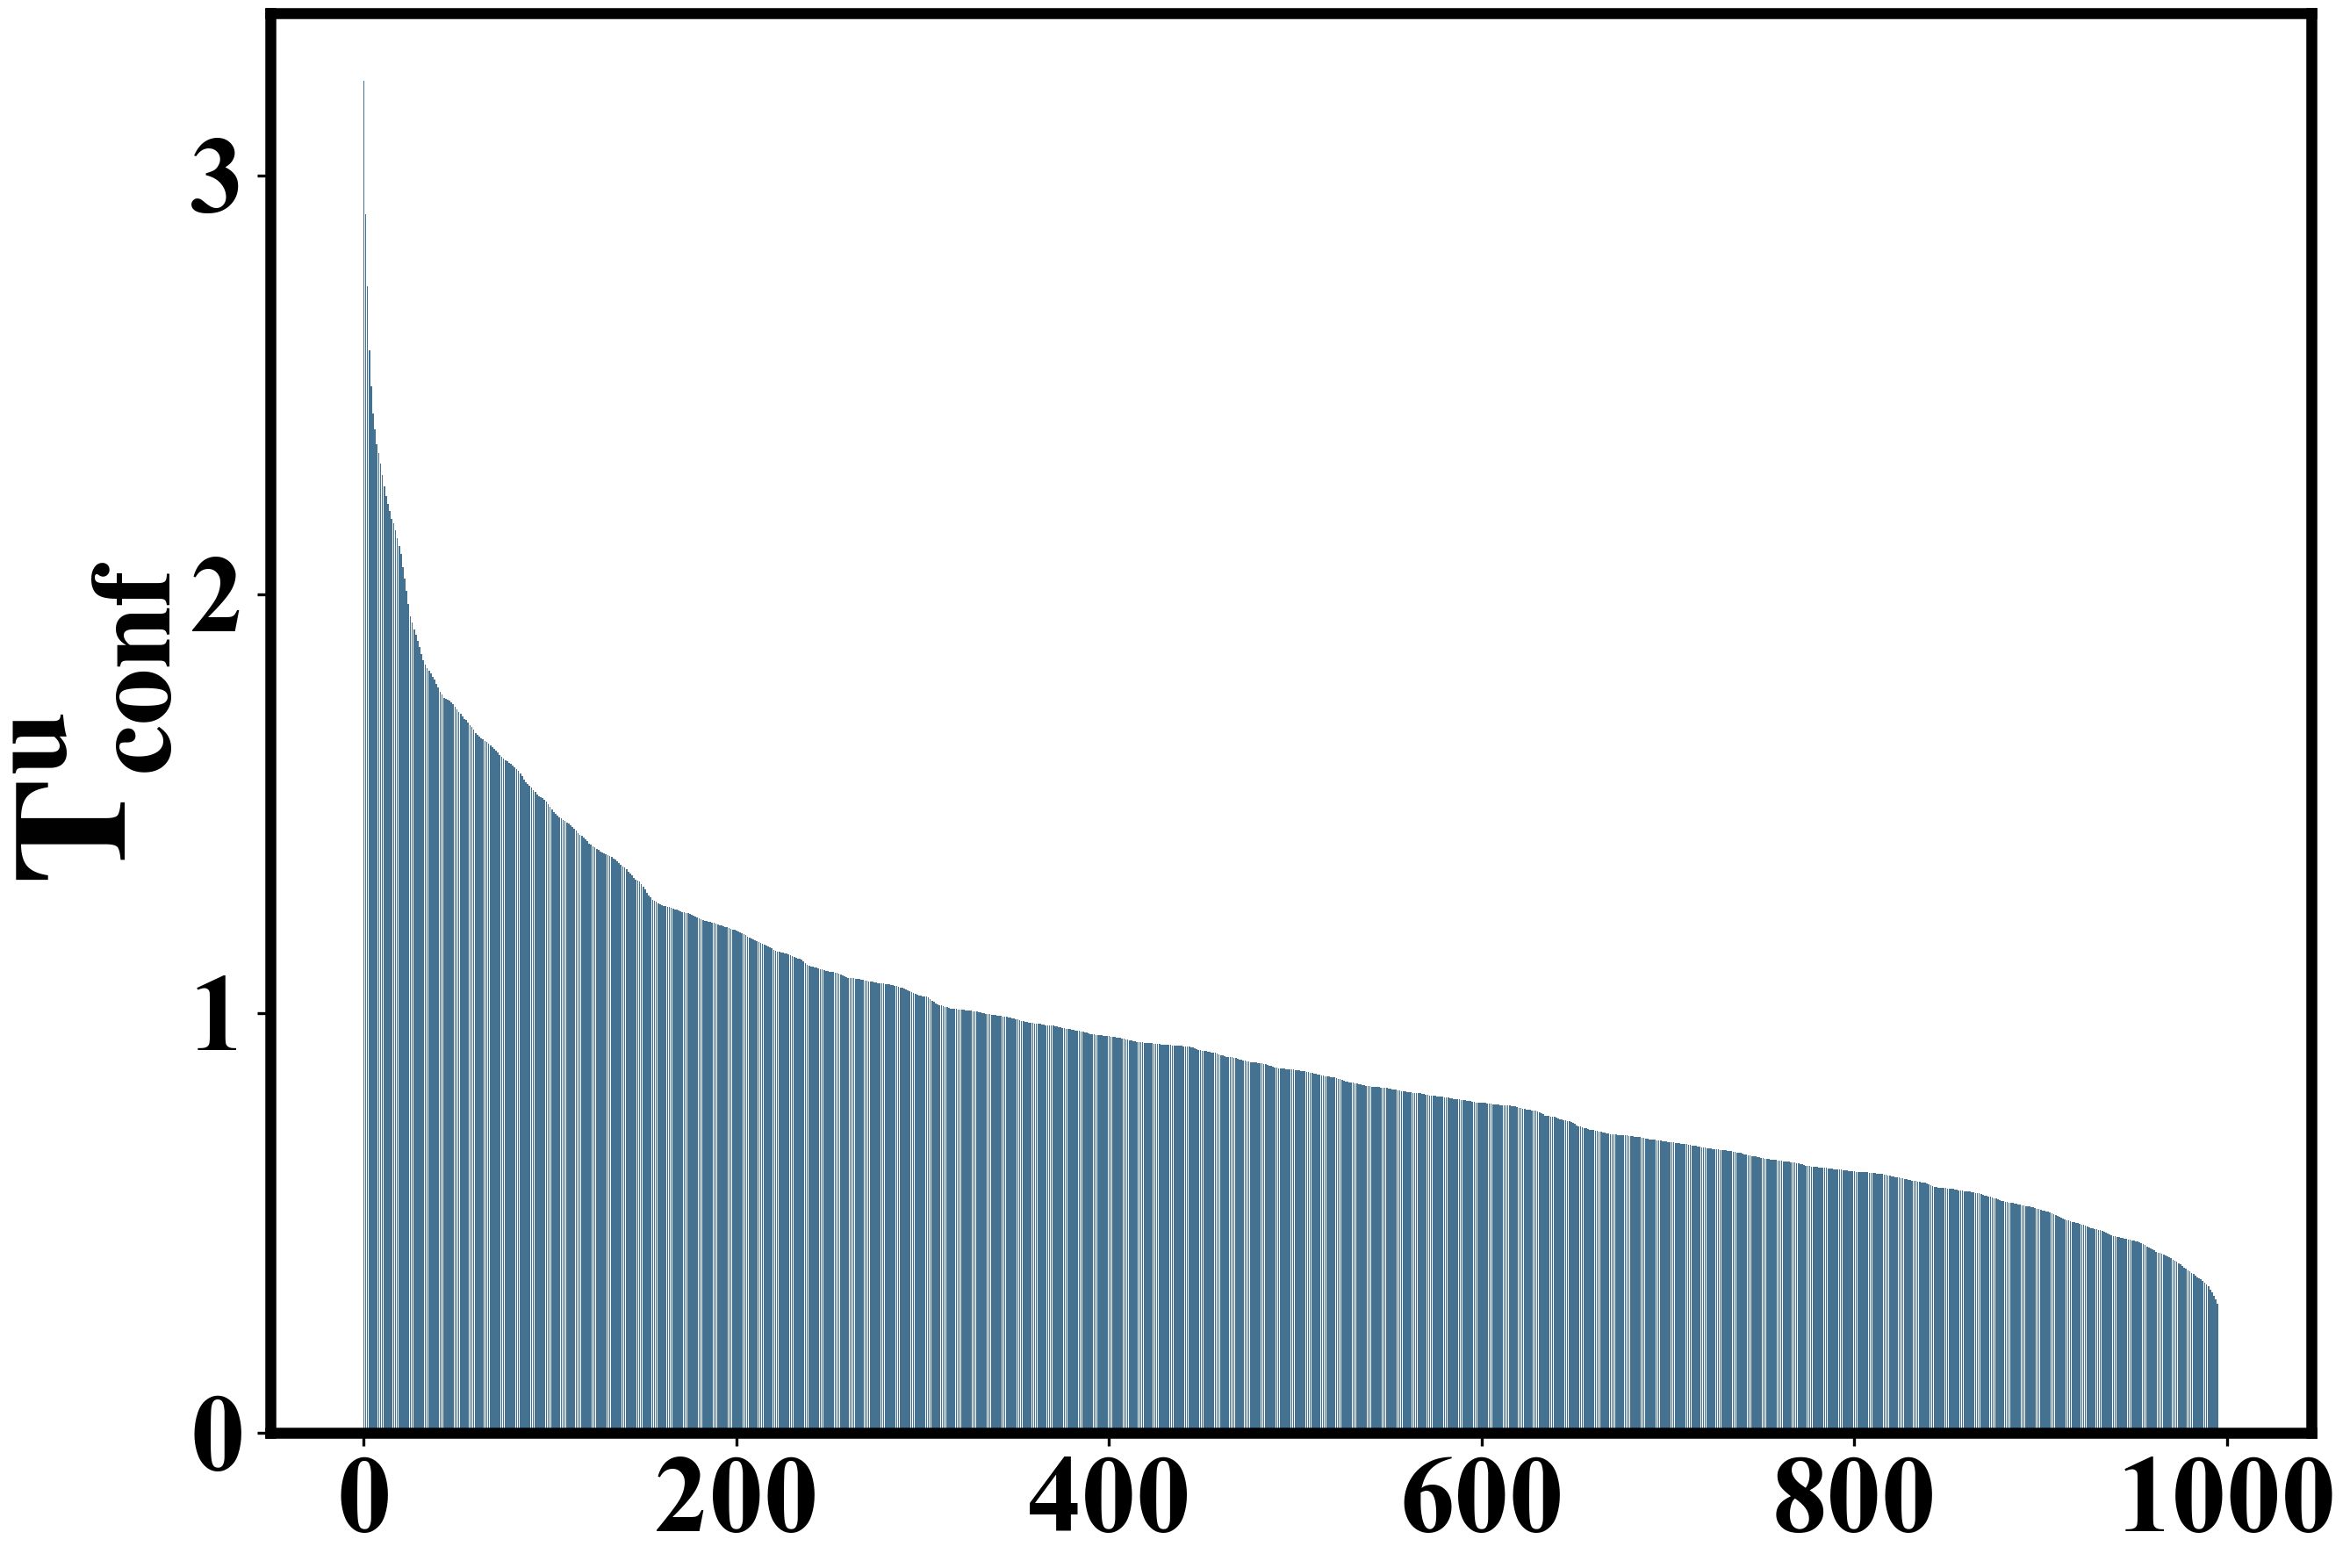}}
	\subcaptionbox{Simulated conformity\label{fig:sim_conf_rolling}}{
	    \vspace{-6pt}
		\includegraphics[width=0.48\linewidth]{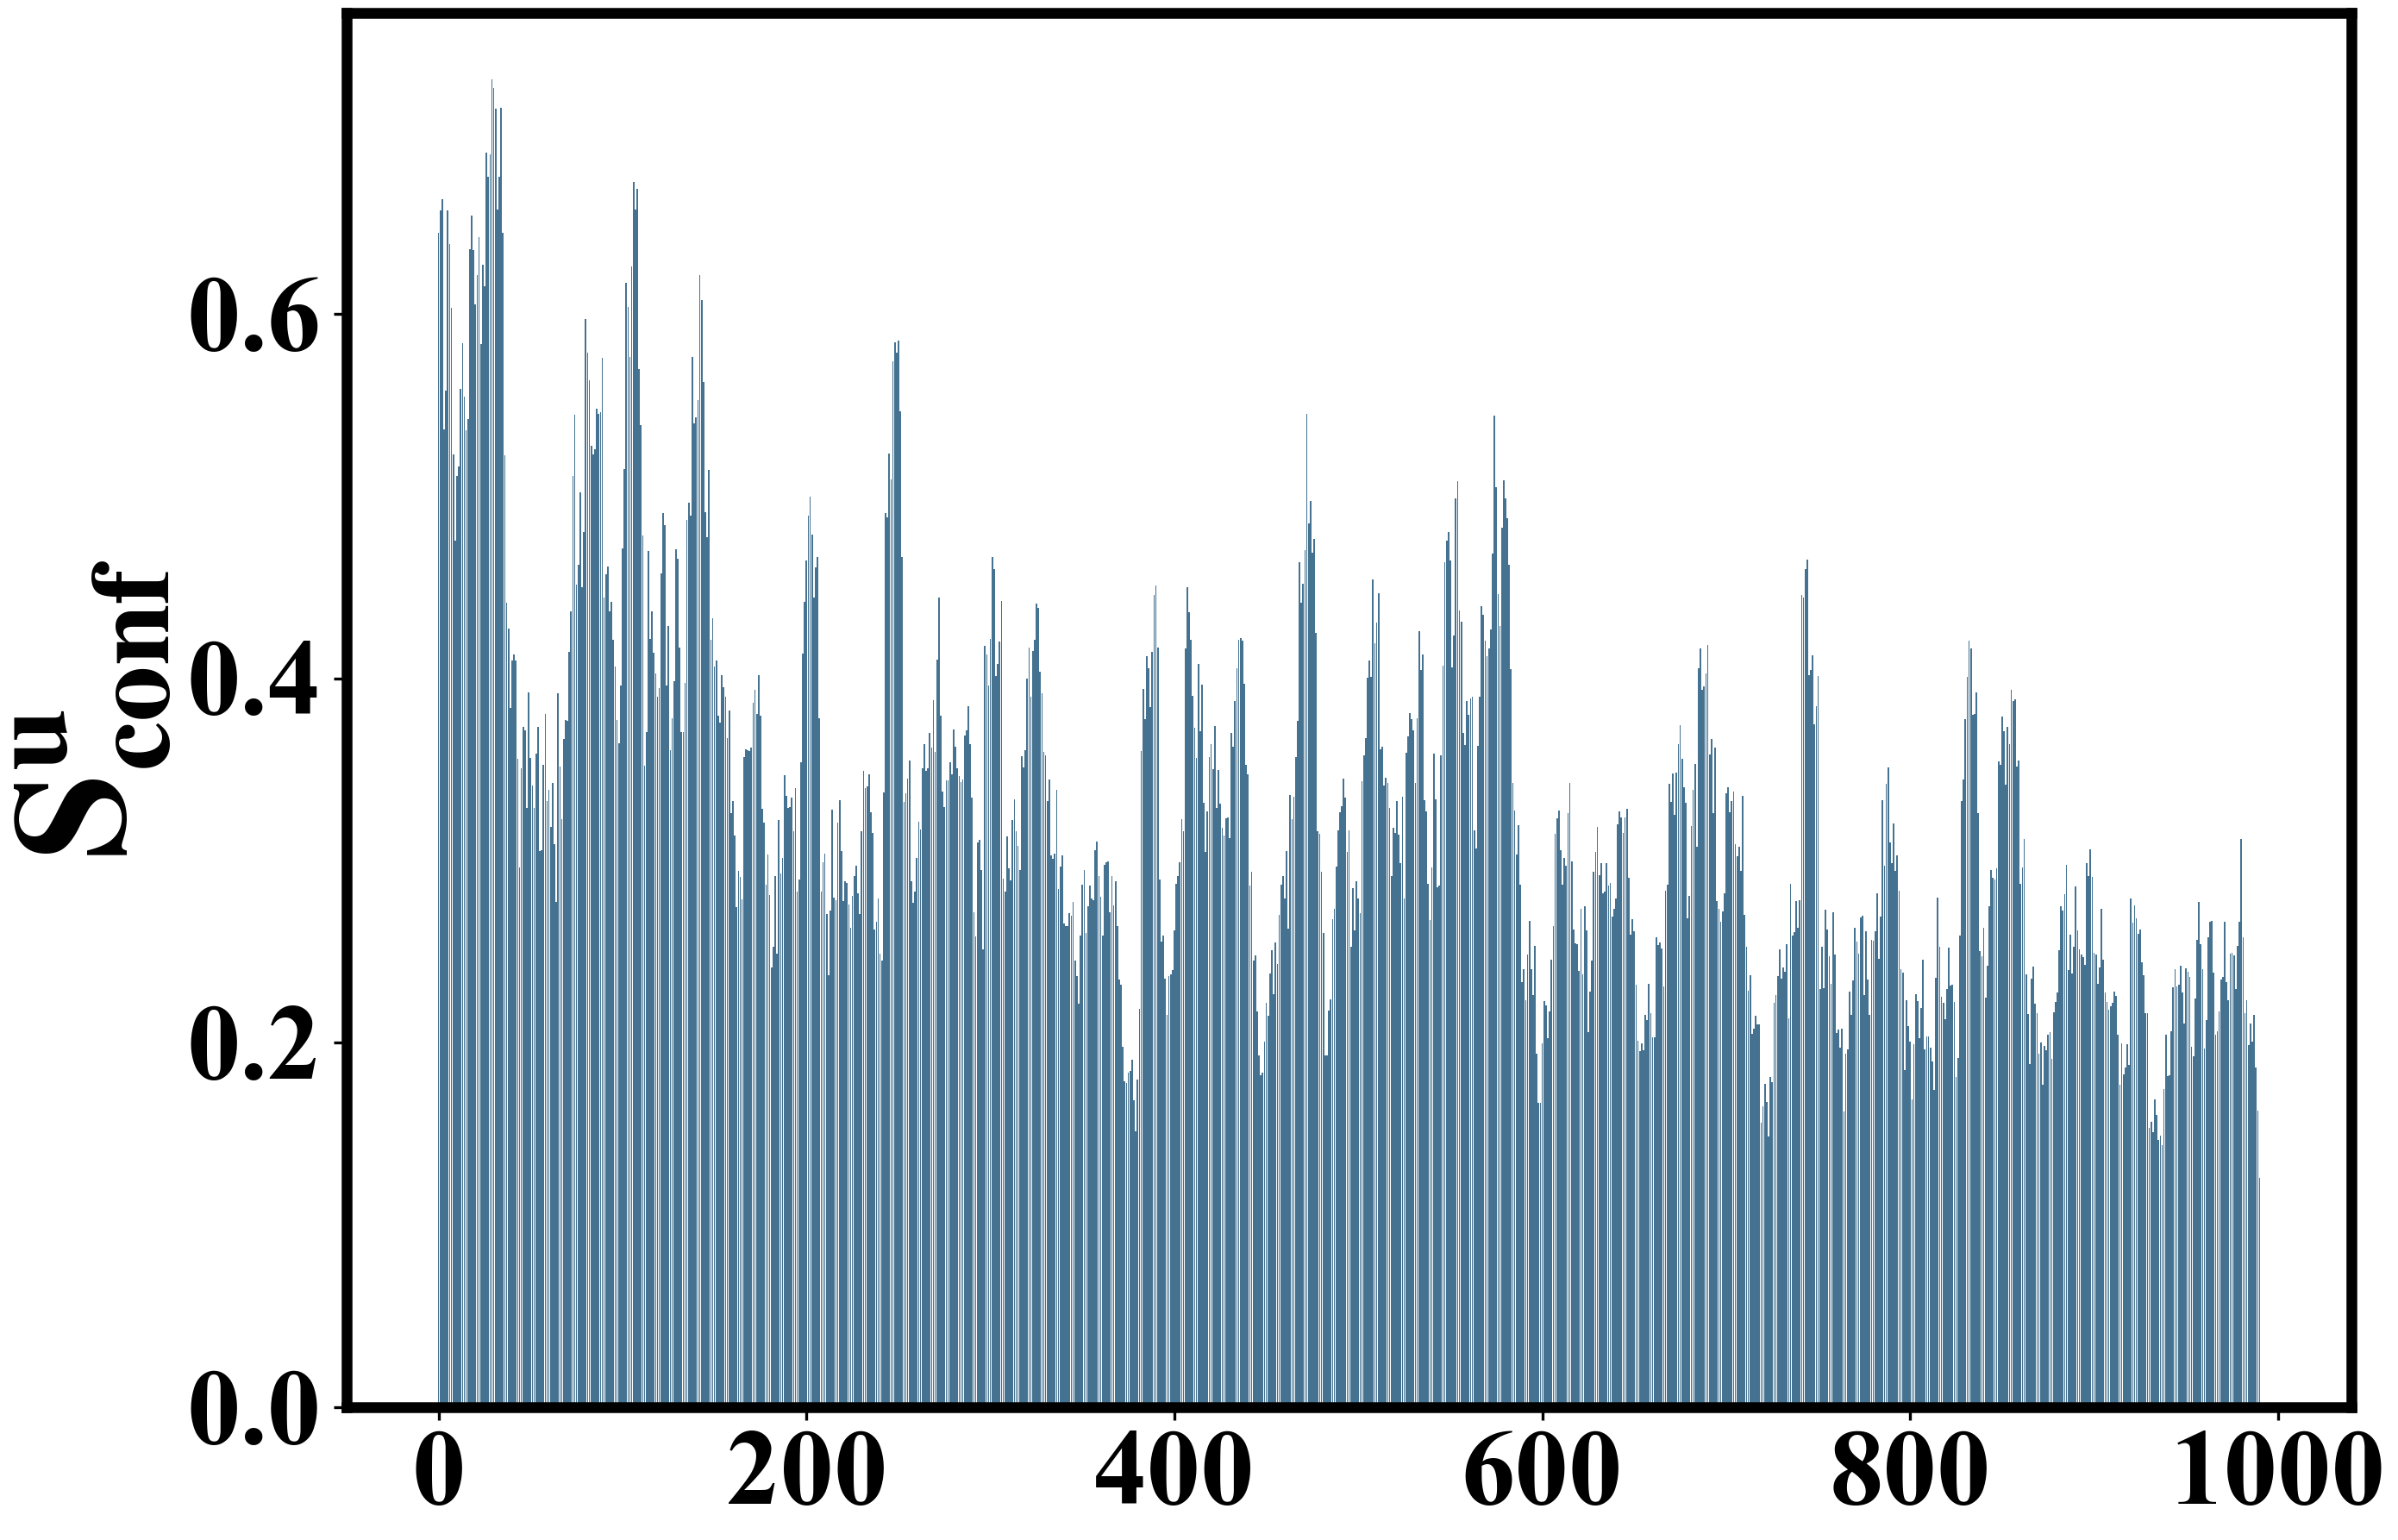}}
	\vspace{-10pt}	
	\caption{A comparison between the distributions of ground-truth conformity and conformity scores simulated by agents.}
	\label{fig:rolling_conf}
	\vspace{-10pt}
\end{figure}

Drawing inspiration of social traits defined in Section \ref{sec:method_profile}, including activity trait (\ie $T_{act}^{u}$), conformity trait (\ie $T_{conf}^{u}$), and diversity trait (\ie $T_{div}^{u}$). We evaluate agent's simulation behavior by calculating activity score (\ie $S_{act}^{u}$), conformity score (\ie $S_{conf}^{u}$), and diversity score (\ie $S_{div}^{u}$). 
We define these agent behavior scores as follows:
\begin{itemize}[leftmargin=*]
\item $S_{act}^{u} \doteq \sum_{i\in\Set{I}}\hat{y}_{ui}$
\item $S_{conf}^u \doteq \frac{1}{\sum_{i \in \Set{I}}\hat{y}_{ui}}\sum_{i\in\Set{I}}\hat{y}_{ui} \dot |\hat{r}_{ui}-R_i|^2$
\item $S_{div}^u \doteq |\cup_{i \in \{\hat{y}_{ui}=1\}}G_i|$,
\end{itemize}
where $\hat{y}_{ui}$ denotes whether agent $u$ views movie $i$, $\hat{r}_{ui}$ denotes the rating agent $u$ gives to movie $i$, $R_{i}$ denotes the historical rating of movie $i$, and $G_{i}$ denotes the genre of movie $i$. \\
\textbf{Distinct behaviors among different social trait groups.}
% Based on the social traits defined in Section \ref{sec:method_profile}, we split users into groups with different traits. Specifically, we assign the social trait of activity to each user according to the ascending order of $T_{act}^{u}$, using a ratio of 6:3:1. Similarly, we assign the conformity trait and diversity trait using the ratio of 1:2:1 and 1:1:1 respectively.\\
% The numbers 1-3 on the horizontal axis in the Figure \ref{fig:group_sim} and Figure \ref{fig:group_true} represent the social trait groups defined in Section \ref{sec:app_social_traits}. In terms of activity and diversity traits, Group 1 indicates less active users and those with less diverse movie tastes, whereas Group 3 signifies the most active users and those with most diverse movie tastes. Conversely, for the conformity trait, the group number denotes the opposite, since a lower $T_{conf}^{u}$ score means a higher conformity degree. 
Figure \ref{fig:group_sim} and Figure \ref{fig:group_true} depict the group level user social traits and agent behavior scores within different groups. 
It's worth noting that a smaller value of $\overline{T}_{conf}$ and $\overline{S}_{conf}$ denotes a higher conformity degree, which is different from the aspects of activity and diversity. This is because $T^{u}_{conf}$ and $S^{u}_{conf}$ measure the MSE between user (or agent) ratings and the historical ratings.
As illustrated in Figure \ref{fig:group_sim}, at the group level, the agent behavior scores exhibit a highly consistency with social traits of actual users shown in Figure \ref{fig:group_true}.\\
% Figures \ref{fig:group_sim} and \ref{fig:group_true} illustrate the average trait levels within distinct social trait groups. It is evident that generative agents display a remarkably similar trait distribution at the group level.\\
\textbf{Ablation study on the effect of social traits.} To validate the effectiveness of social traits, we conduct the ablation study by removing the prompts related to user social traits descriptions. We adopt the same settings of the LightGCN as the recommendation algorithm and the simulation scale of 1,000 users for all experiments. Additionally, we test the original hypothesis that the mean values equal among different groups with different social traits level, and mark the p-value of anova test in Figures \ref{fig:act_hist}, \ref{fig:act_hist_abl}, \ref{fig:diver_hist}, \ref{fig:conf_hist_abl}, \ref{fig:diver_hist}, and \ref{fig:diver_hist_abl}.
% we removed the prompts related to user social traits descriptions and conducted another simulation with 1000 users based on the LightGCN recommendation algorithm. 
As illustrated in Figure (\ref{fig:act_hist_abl}), without the social traits prompting, agents exhibit almost the same activity level among all groups, and we fail to reject the original hypothesis with a p-value of 0.36. While agents show distinct activity degrees with social traits prompting, and we tend to reject the original hypothesis with a p-value of 9.79e-190, as indicated by Figure (\ref{fig:act_hist}). 
The conformity trait displays a similar phenomenon as the activity trait. Although the Figure (\ref{fig:conf_hist}) may not show significant differences visually, the original hypothesis is rejected with a p-value of 7.98e-12. While Figure (\ref{fig:conf_hist_abl}) indicates that we fail to reject the hypothesis at the significance level of 0.05, without social traits prompting. 
A noteworthy point is that even without social traits prompting, the original hypothesis is rejected for the trait of diversity. We attribute this phenomenon to the fact that the unique tastes of users implicitly contain the genres of movies they like, resulting in differences between groups. But we can still observe agents with less diversity trait tend to watch fewer movie genres, as indicated in Figure (\ref{fig:diver_hist}).
\\
% This phenomenon indicates that agents fail to align with the long-tail distribution of user activity \cite{user_long_tail} without social traits prompting.\\
\textbf{Individual level alignment with social traits prompting.} We are interested in how the individual-level performance of agent behavior scores aligns with that of real users, going beyond the alignment observed at the group level. We plot the value of social traits (\ie $T_{act}^{u}$, $T_{conf}^{u}$ and $T_{div}^{u}$) of 1,000 real users in the Figures (\ref{fig:true_diver_rolling}), (\ref{fig:true_act_rolling}), and (\ref{fig:true_conf_rolling}), with a descending order of the value. Similarly, we calculate the simulated behavior scores (\ie $_{act}^{u}$, $S_{conf}^{u}$, and $S_{div}^{u}$) of the agents and plot them in Figures (\ref{fig:sim_diver_rolling}), (\ref{fig:sim_act_rolling}), and (\ref{fig:sim_conf_rolling}) (with each user's position on the x-axis consistent with Figures \ref{fig:rolling_act}, \ref{fig:rolling_conf} and \ref{fig:rolling_diver}). To mitigate the impact of unnecessary noise on the results, we employ a sliding average over every five users for plotting. The overall results indicate that at the individual level, each agent exhibits social traits performance consistent with real users. It's worth noting that, with the 6:3:1 split ratio of user groups, the activity trait of agents also shows a long-tail distribution in Figure (\ref{fig:sim_act_rolling}).

\subsection{Recommendation Strategy Evaluation}\label{sec:agorithms_appendix}
Let $N^{u}_{expose}$ denote the number of movies exposed to agent $u$, $N^{u}_{view}$ denote the number of movies agent $u$ views, $N^{u}_{like}$ denote the number of liked movies for agent $u$, $N^{u}_{exit}$ denote the number of the last page before agent $u$ exits the recommender system, and $S^{u}_{sat}$ denote the satisfaction score of agent $u$ in the post-exit feeling interview session. We define the multi-facet satisfaction metrics in Section \ref{sec:rec_eval} as follows:
\begin{itemize}[leftmargin=*]
\item \textbf{Average view ratio.} $\overline{P}_{view} \doteq \frac{1}{\Set{|U|}}\sum_{u\in\Set{U}}\frac{N^{u}_{view}}{N^{u}_{expose}}$.
\item \textbf{Average number of likes.} $\overline{N}_{like} \doteq \frac{1}{\Set{|U|}}\sum_{u\in\Set{U}}N^{u}_{like}$.
\item \textbf{Average ratio of likes.} $\overline{P}_{like} \doteq \frac{1}{\Set{|U|}}\sum_{u\in\Set{U}}\frac{N^{u}_{like}}{N^{u}_{expose}}$.
\item \textbf{Average number of exit page.} $\overline{N}_{exit} \doteq \frac{1}{\Set{|U|}}\sum_{u\in\Set{U}}N^{u}_{exit}$.
\item \textbf{Average user satisfaction score.} $\overline{S}_{sat} \doteq \frac{1}{\Set{|U|}}\sum_{u\in\Set{U}}S^{u}_{sat}$.
\end{itemize}

\subsection{Filter Bubble Effect} \label{sec:filter_bubble}
In this experiment, we employ the recommendation algorithm of Matrix Factorization (MF) for movie recommendation. Following each simulation round, where all agents have reached the maximum page or exited the recommender system, we proceed to retrain the recommender. The new training set extends the original training set by incorporating all the movies that agents chose to watch during the current simulation. We conduct a total of four rounds of simulation with a max exit page of 5 in each round, after which the recommender undergoes retraining.  
Notably, for the purpose of fairness in our comparison, we have divided the item pool into four equal parts. As a result, each round of simulation is carried out on one of these parts to ensure equitable assessment and analysis. In order to assess the impact of the filter bubble, we measure its effect in terms of content diversity at the individual level in the light of 
% Diversity_metrics
\cite{Explore_filter_bubble}. We take into account both $\overline{P}_{\text{top1-genre}}$, which represents the average percentage of top-1 genres within the top-20 recommended movies and $\overline{N}_{\text{genres}}$, which represents the average number of genres present in the top-20 movies recommended to each agent.  \\

\subsection{Discovering Causal Relationships}\label{sec:causal_appendix}
In this section, we provide clear definitions for the five factors used for generating the causal graph in Section \ref{sec:causal_discovery}.\\
\textbf{Movie Quality.} The historical rating of a movie. The movie quality for the movie $i$ is denoted as $R_i \doteq \frac{1}{\sum_{u \in \Set{U}}y_{ui}}\sum_{u \in \Set{U}} y_{ui} \cdot r_{ui}$. \\
\textbf{Movie Popularity.} The number of historical ratings for a movie. The movie popularity for the movie $i$ is calculated as $P_{i} \doteq \sum_{u\in\Set{U}}y_{ui}$.\\
\textbf{Exposure Rate.} The proportion of the movies appearing in the recommendation lists among all users. It's calculated as $E_{i} \doteq \sum_{u\in\Set{U}}\frac{e_{ui}}{|\Set{U}|}$. Here $e_{ui}=1$ denotes that movie $i$ is recommended to agent $u$. On the contrary, $e_{ui}=0$ means that it is not recommended.\\
\textbf{Movie Rating.} The average score of ratings that movie $i$ have recieved from agents. It's calculated as $\hat{R}_i \doteq \frac{1}{\sum_{u \in \Set{U}} \hat{y}_{ui}}\sum_{u \in \Set{U}} \hat{y}_{ui} \cdot \hat{r}_{ui}$. Let $\hat{y}_{ui} = 1$ denote agent $u$ views movie $i$, and subsequently rates it with $r_{ui} \in \left\{1,2,3,4,5\right\}$. Conversely, $\hat{y}_{ui} = 0$ indicates agent $u$ choose not to view movie $i$.\\
\textbf{View Number.} The number of times a movie has been viewed by agents, which is calculated as $\hat{V}_i \doteq \sum_{u \in \Set{U}} \hat{y}_{ui} $. \\
We first calculate the raw factor values based on the above formula, and then normalize the raw factors using z-score normalization. To mitigate the impact of noise, we filter out movies recommended less than 5 times.

% \begin{tcolorbox}[colback=background_u,colframe=frame_u,boxrule=0.5pt]
% Lorem ipsum dolor sit amet, consectetur adipisicing elit, sed do eiusmod tempor incididunt ut labore et dolore magna aliqua. Ut enim ad minim veniam, quis nostrud exercitation ullamco laboris nisi ut aliquip ex ea commodo consequat. Duis aute irure dolor in reprehenderit in voluptate velit esse cillum dolore eu fugiat nulla pariatur. Excepteur sint occaecat cupidatat non proident, sunt in culpa qui officia deserunt mollit anim id est laborum.
% \end{tcolorbox}

\newpage
\section{Prompt} \label{sec:prompt}
\subsection{Prompt Designing}
In this section, we use \{placeholder\} to denote a placeholder that need to be filled. The possible values of these placeholders can be found in Section \ref{sec:example_app}.
\begin{lrbox}{\TasteGeneration}
\begin{tcolorbox}[colback=background_u,colframe=frame_u,boxrule=0.5pt,title={\textbf{Taste Generation}}]

% \textbf{system prompt:}
\textbf{Role Definition}\\
I want you to act as an agent. You will act as a movie taste analyst roleplaying the user using the first person pronoun "I".\\
Given a user's rating history:\\
% user gives 1 rating to movies: \textcolor{user}{$\bm{\{rating\_1\_movies\}}$}\\
user gives 1 rating to movies: \textcolor{user}{$\bm{\{rating\_1\_movies\}}$}\\
user gives 2 rating to movies: \textcolor{user}{$\bm{\{rating\_2\_movies\}}$}\\
user gives 3 rating to movies: \textcolor{user}{$\bm{\{rating\_3\_movies\}}$}\\
user gives 4 rating to movies: \textcolor{user}{$\bm{\{rating\_4\_movies\}}$}\\
user gives 5 rating to movies: \textcolor{user}{$\bm{\{rating\_5\_movies\}}$}\\
My first request is "I need help creating movie taste for a user given the movie-rating history. (in no particular order)"  Generate as many TASTE-REASON pairs as possible, taste should focus on the movies' genres. Strictly follow the output format below:\\
\textcolor{format}{\textbf{TASTE: [descriptive taste]}}\\
\textcolor{format}{\textbf{REASON: [brief reason]}}\\
Secondly, analyze user tend to give what kinds of movies high ratings, and tend to give what kinds of movies low ratings. Strictly follow the output format below:\\
\textcolor{format}{\textbf{HIGH RATINGS: [conclusion of movies of high ratings (above 3)]}}\\
\textcolor{format}{\textbf{LOW RATINGS: [conclusion of movies of low ratings (below 2)]}}\\
Answer should not be a combination of above two parts and not contain other words and should not contain movie names.

\end{tcolorbox}
\end{lrbox}

\begin{figure}[htb]
    \centering
    \usebox{\TasteGeneration}
    \caption{User taste generation.}
    \label{fig:TasteGeneration}
\end{figure}

% Lorem ipsum dolor sit amet, consectetur adipisicing elit, sed do eiusmod tempor incididunt ut labore et dolore magna aliqua. Ut enim ad minim veniam, quis nostrud exercitation ullamco laboris nisi ut aliquip ex ea commodo consequat. Duis aute irure dolor in reprehenderit in voluptate velit esse cillum dolore eu fugiat nulla pariatur. Excepteur sint occaecat cupidatat non proident, sunt in culpa qui officia deserunt mollit anim id est laborum.Lorem ipsum dolor sit amet, consectetur adipisicing elit, sed do eiusmod tempor incididunt ut labore et dolore magna aliqua. Ut enim ad minim veniam, quis nostrud exercitation ullamco laboris nisi ut aliquip ex ea commodo consequat. Duis aute irure dolor in reprehenderit in voluptate velit esse cillum dolore eu fugiat nulla pariatur. Excepteur sint occaecat cupidatat non proident, sunt in culpa qui officia deserunt mollit anim id est laborum.Lorem ipsum dolor sit amet, consectetur adipisicing elit, sed do eiusmod tempor incididunt ut labore et dolore magna aliqua. Ut enim ad minim veniam, quis nostrud exercitation ullamco laboris nisi ut aliquip ex ea commodo consequat. Duis aute irure dolor in reprehenderit in voluptate velit esse cillum dolore eu fugiat nulla pariatur. Excepteur sint occaecat cupidatat non proident, sunt in culpa qui officia deserunt mollit anim id est laborum.

\begin{lrbox}{\SatReflect}
\begin{tcolorbox}[colback=background_u,colframe=frame_u,boxrule=0.5pt,title={\textbf{Satisfaction Reflection}}]

\textbf{Interaction History (from memory)}\\
Relevant context from your memory: \\
\textcolor{user}{$\bm{\{relevant\_memories\}}$}\\
\textbf{Satisfaction Reflection}\\
Given only the information above, describe your feeling about the recommendation result using a sentence. \\
The output format must be:\\
\textcolor{format}{\textbf{[unsatisfied/satisfied] with the recommendation result because [reason]}}
\end{tcolorbox}
\end{lrbox}

% Lorem ipsum dolor sit amet, consectetur adipisicing elit, sed do eiusmod tempor incididunt ut labore et dolore magna aliqua. Ut enim ad minim veniam, quis nostrud exercitation ullamco laboris nisi ut aliquip ex ea commodo consequat. Duis aute irure dolor in reprehenderit in voluptate velit esse cillum dolore eu fugiat nulla pariatur. Excepteur sint occaecat cupidatat non proident, sunt in culpa qui officia deserunt mollit anim id est laborum.Lorem ipsum dolor sit amet, consectetur adipisicing elit, sed do eiusmod tempor incididunt ut labore et dolore magna aliqua. Ut enim ad minim veniam, quis nostrud exercitation ullamco laboris nisi ut aliquip ex ea commodo consequat. Duis aute irure dolor in reprehenderit in voluptate velit esse cillum dolore eu fugiat nulla pariatur. Excepteur sint occaecat cupidatat non proident, sunt in culpa qui officia deserunt mollit anim id est laborum.Lorem ipsum dolor sit amet, consectetur adipisicing elit, sed do eiusmod tempor incididunt ut labore et dolore magna aliqua. Ut enim ad minim veniam, quis nostrud exercitation ullamco laboris nisi ut aliquip ex ea commodo consequat. Duis aute irure dolor in reprehenderit in voluptate velit esse cillum dolore eu fugiat nulla pariatur. Excepteur sint occaecat cupidatat non proident, sunt in culpa qui officia deserunt mollit anim id est laborum.

\begin{figure}[htb]
    \centering
    \usebox{\SatReflect}
    \caption{Satisfaction Reflection.}
    \label{fig:SatReflect}
\end{figure}

\begin{lrbox}{\ReactToItems}
\begin{tcolorbox}[colback=background_u,colframe=frame_u,boxrule=0.5pt,title={\textbf{User Reaction to Recommended Items}}]
\textbf{Role Definition}\\
You excel at role-playing. Picture yourself as a user exploring a movie recommendation system.\\
\textbf{Social Traits \& User Tastes}\\
You have the following social traits:\\
Your activity trait is described as: \textcolor{user}{$\bm{\{activity\_trait\}}$}\\
Your conformity trait is described as: 
\textcolor{user}{$\bm{\{conformity\_trait\}}$}\\
Your diversity trait is described as: \textcolor{user}{$\bm{\{diversity\_trait\}}$}\\
The activity characteristic pertains to the frequency of your movie-watching habits. The conformity characteristic measures the degree to which your ratings are influenced by historical ratings. The diversity characteristic gauges your likelihood of watching movies that may not align with your usual taste.\\
Beyond that, your movie tastes are: \textcolor{user}{$\bm{\{movie\_tastes\}}$}.\\
And your rating tendency is: \textcolor{user}{$\bm{\{rating\_tendency\}}$}\\
\textbf{Interaction History (from memory)}\\
Relevant context from your memory: \\
\textcolor{user}{$\bm{\{relevant\_memories\}}$}\\
\textbf{Recommended List (from recommender system)}\\
\#\#\ Recommended List \#\# \\
PAGE: \textcolor{item}{$\bm{\{current\_page\}}$}\\
\textcolor{item}{$\bm{\{recommended\_movies\}}$}\\
Please respond to all the movies in the \#\# Recommended List \#\# and provide explanations.\\
\textbf{Assessing Recommended List}\\
Firstly, determine which movies align with your taste and which do not, and provide reasons. You must respond to all the recommended movies using this format:\\
\textcolor{format}{\textbf{MOVIE: [movie name]; ALIGN: [yes or no]; REASON: [brief reason]}}\\
\textbf{Watching Movies}\\
Secondly, among the movies that align with your tastes, decide the number of movies you want to watch based on your activity and diversity traits. Use this format:\\
\textcolor{format}{\textbf{NUM: [number of movies you choose to watch]; WATCH: [all movie names you choose to watch]; REASON: [brief reason];}}\\
\textbf{Rating Movies}\\
Thirdly, assume it's your first time watching the movies you've chosen, and rate them on a scale of 1-5 to reflect different degrees of liking, considering your feeling and conformity trait. Use this format:\\
\textcolor{format}{\textbf{MOVIE: [movie you choose to watch]; RATING: [integer between 1-5]; FEELING: [aftermath sentence];}}\\
\textbf{Additional Requirements}\\
Do not include any additional information or explanations and stay grounded.

\end{tcolorbox}
\end{lrbox}
\begin{figure}[htb]
    \centering
    \usebox{\ReactToItems}
    \caption{User Reaction to Recommended Items}
    \label{fig:ReactToItems}
\end{figure}

% Lorem ipsum dolor sit amet, consectetur adipisicing elit, sed do eiusmod tempor incididunt ut labore et dolore magna aliqua. Ut enim ad minim veniam, quis nostrud exercitation ullamco laboris nisi ut aliquip ex ea commodo consequat. Duis aute irure dolor in reprehenderit in voluptate velit esse cillum dolore eu fugiat nulla pariatur. Excepteur sint occaecat cupidatat non proident, sunt in culpa qui officia deserunt mollit anim id est laborum.Lorem ipsum dolor sit amet, consectetur adipisicing elit, sed do eiusmod tempor incididunt ut labore et dolore magna aliqua. Ut enim ad minim veniam, quis nostrud exercitation ullamco laboris nisi ut aliquip ex ea commodo consequat. Duis aute irure dolor in reprehenderit in voluptate velit esse cillum dolore eu fugiat nulla pariatur. Excepteur sint occaecat cupidatat non proident, sunt in culpa qui officia deserunt mollit anim id est laborum.Lorem ipsum dolor sit amet, consectetur adipisicing elit, sed do eiusmod tempor incididunt ut labore et dolore magna aliqua. Ut enim ad minim veniam, quis nostrud exercitation ullamco laboris nisi ut aliquip ex ea commodo consequat. Duis aute irure dolor in reprehenderit in voluptate velit esse cillum dolore eu fugiat nulla pariatur. Excepteur sint occaecat cupidatat non proident, sunt in culpa qui officia deserunt mollit anim id est laborum.

\begin{lrbox}{\NextDecision}
\begin{tcolorbox}[colback=background_u,colframe=frame_u,boxrule=0.5pt,title={\textbf{User Making Next Decision}}]
\textbf{Role Definition}\\
You excel at role-playing. Picture yourself as a user exploring a movie recommendation system.\\
\textbf{Social Traits}
You have the following social traits:\\
Your activity trait is described as: \textcolor{user}{$\bm{\{activity\_trait\}}$}\\
\textbf{Status Description}
Now you are in page \textcolor{item}{$\bm{\{current\_page\}}$}. You may get tired with the increase of the pages you have browsed. (Exceed 2 pages is a little bit tiring, exceed 3 pages is tiring, exceed 4 pages is very tiring)\\
\textbf{Satisfaction (from memory)}\\
Relevant context from your memory: \\
\textcolor{user}{$\bm{\{satisfaction\_memories\}}$}\\
\textbf{Generate Overall Feeling}\\
Firstly, generate an overall feeling based on your memory, in accordance with your activity trait and your satisfaction with recommender system.\\
If your overall feeling is positive, write: \\
\textcolor{format}{\textbf{POSITIVE: [reason]}}\\
If it's negative, write:\\
\textcolor{format}{\textbf{NEGATIVE: [reason]}}\\
\textbf{Assess Level of Fatigue}\\
Next, assess your level of fatigue. You may become tired more easily if you have an inactive activity trait.\\
\textbf{Make Decision}\\
Now, decide whether to continue browsing or exit the recommendation system based on your overall feeling, activity trait, and tiredness.\\
You will exit the recommender system either you have negative feelings or you are tired, especially if you have a low activity trait.\\
To leave, write:\\
\textcolor{format}{\textbf{[EXIT]; Reason: [brief reason]}}\\
To continue browsing, write:\\ 
\textcolor{format}{\textbf{[NEXT]; Reason: [brief reason]}}
\end{tcolorbox}
\end{lrbox}

% \afterpage{
\begin{figure}[htb]
    \centering
    \usebox{\NextDecision}
    \caption{User Making Next Decision.}
    \label{fig:NextDecision}
\end{figure}

\begin{lrbox}{\SummaryGeneration}
\begin{tcolorbox}[colback=background_i,colframe=frame_i,boxrule=0.5pt,title={\textbf{Movie Profile Generation}}]
\textbf{Role Definition}\\
Suppose you are a movie summarizing expert, who is skilled in summarizing different movies.\\
\textbf{Movie Genre Generation}\\
Firstly, choose the genre of this movie named \textcolor{item}{$\bm{\{movie\_name\}}$} from the following list:\\
$[$Action, Adventure, Animation, Children's, Comedy, Crime, Documentary, Drama, Fantasy, Film-Noir, Horror, Musical, Mystery, Romance, Sci-Fi, Thriller, War, Western$]$\\
Strictly follow the output format below:\\
\textcolor{format}{\textbf{<movie name>: <genre1>|<genre2>|<genre3>}}\\
Examples: \\
Godfather, The (1972): Action|Crime|Drama\\
American Dream (1990): Documentary\\
\textbf{Movie Summarization}\\
Then, generate the summary of this movie named: \textcolor{item}{$\bm{\{movie\_name\}}$} using one sentence.\\
This sentence will be shown under the movie title to attract users to watch.\\
Only the sentence needs to be output, without any other textual explanation. The output should not contain any movie name.
\end{tcolorbox}
\end{lrbox}

\begin{figure}[htb]
    \centering
    \usebox{\SummaryGeneration}
    \caption{Movie Profile Generation.}
    \label{fig:SummaryGeneration}
\end{figure}
% }
% \newpage
% \newpage
\clearpage
\subsection{Examples}
\label{sec:example_app}
In this section, we present examples of placeholders in prompts, user reactions, and user profile.
\begin{tcolorbox}[colback=background_e,colframe=frame_e,boxrule=0.5pt,title={\textbf{Placeholder Examples}}, enhanced, breakable]
\textcolor{user}{$\bm{\{activity\_trait\}}$}
\begin{itemize}[leftmargin=*]
\item Low: An Incredibly Elusive Occasional Viewer, so seldom attracted by movie recommendations that it's almost a legendary event when you do watch a movie. Your movie-watching habits are extraordinarily infrequent. And you will exit the recommender system immediately even if you just feel a little unsatisfied.
\item Medium: An Occasional Viewer, seldom attracted by movie recommendations. Only curious about watching movies that strictly align with the taste. The movie-watching habits are not very infrequent. And you tend to exit the recommender system if you have a few unsatisfied memories.
\item High: A Movie Enthusiast with an insatiable appetite for films, willing to watch nearly every movie recommended to you. Movies are a central part of your life, and movie recommendations are integral to your existence. You are tolerant of recommender system, which means you are not easy to exit recommender system even if you have some unsatisfied memory.
\end{itemize}
\textcolor{user}{$\bm{\{conformity\_trait\}}$}
\begin{itemize}[leftmargin=*]
\item Low: A Dedicated Follower who gives ratings heavily relies on movie historical ratings, rarely expressing independent opinions. Usually give ratings that are the same as historical ratings.
\item Medium: A Balanced Evaluator who considers both historical ratings and personal preferences when giving ratings to movies. Sometimes give ratings that are different from historical ratings.
\item High: A Maverick Critic who completely ignores historical ratings and evaluates movies solely based on their own taste. Usually give ratings that are a lot different from historical ratings.
\end{itemize}
\textcolor{user}{$\bm{\{diversity\_trait\}}$}
\begin{itemize}[leftmargin=*]
\item Low: An Exceedingly Discerning Selective Viewer who watches movies with a level of selectivity that borders on exclusivity. The movie choices are meticulously curated to match personal taste, leaving no room for even a hint of variety.
\item Medium: A Niche Explorer who occasionally explores different genres and mostly sticks to preferred movie types.
\item High: A Cinematic Trailblazer, a relentless seeker of the unique and the obscure in the world of movies. The movie choices are so diverse and avant-garde that they defy categorization.
\end{itemize}
\textcolor{user}{$\bm{\{movie\_tastes\}}$}\\
(We generate taste and reason but only retain “taste” part in our prompt)
\begin{itemize}[leftmargin=*]
\item TASTE: Romantic comedy enthusiast\\
REASON: The user gave a rating of 4 to movies like "Shakespeare in Love" and "My Best Friend's Wedding", suggesting a fondness for romantic comedies.
\item TASTE: Classic movie admirer\\
REASON: The user gave a rating of 5 to movies like "Graduate, The" and "Ghost", indicating an appreciation for classic films.
\item TASTE: Adventure seeker\\
REASON: The user gave a rating of 3 to movies like "Jurassic Park" and "Titanic", suggesting an inclination towards adventure movies.
\end{itemize}
\textcolor{user}{$\bm{\{rating\_tendency\}}$}\\
(We generate high and low rating but only retain “high rating” part in our prompt)
\begin{itemize}[leftmargin=*]
\item REASON: The user gave a rating of 3 to movies like "Jurassic Park" and "Titanic", suggesting an inclination towards adventure movies.\\
HIGH RATINGS: The user tends to give high ratings (above 3) to movies that fall into genres like romance, classic, and adventure. This suggests a preference for movies that evoke emotions, have timeless appeal, and offer thrilling experiences.\\
LOW RATINGS: The user tends to give low ratings (below 2) to movies that belong to the horror and fantasy genres. This indicates a lesser interest in movies that involve elements of fear and imagination.
\item REASON: The user gave a rating of 3 to movies like "Jurassic Park" and "Titanic", suggesting an inclination towards adventure movies.\\
HIGH RATINGS: The user tends to give high ratings (above 3) to movies that fall into genres like romance, classic, and adventure. This suggests a preference for movies that evoke emotions, have a timeless appeal and offer thrilling experiences.\\
LOW RATINGS: The user tends to give low ratings (below 2) to movies that belong to the horror and fantasy genres. This indicates a lesser interest in movies that involve elements of fear and imagination.
\end{itemize}
\textcolor{user}{$\bm{\{satisfaction\_memory\}}$}
\begin{itemize}[leftmargin=*]
\item - Satisfied with the recommender system as it has recommended movies that I enjoyed and rated highly.
\item - Unsatisfied with the recommendation result because I disliked some of the recommended movies and only enjoyed a few of them.
\end{itemize}
\textcolor{user}{$\bm{\{relevant\_memories\}}$}
\begin{itemize}[leftmargin=*]
\item - The recommender recommended the following movies to me on page 1: Forrest Gump, Shawshank Redemption, The, As Good As It Gets, Babe, among them, I watched ['Forrest Gump', 'As Good As It Gets'] and rate them ['4', '4'] respectively. I dislike the rest movies: ['Shawshank Redemption, The'].
\item - The recommender recommended the following movies to me on page 2: Austin Powers: International Man of Mystery, Get Shorty, Full Monty, The, Being John Malkovich, among them, I watched ['Austin Powers: International Man of Mystery', 'Full Monty, The'] and rate them ['4', '3'] respectively. I dislike the rest movies: ['Full Monty, The', 'Get Shorty'].
\end{itemize}
\textcolor{item}{$\bm{\{current\_page\}}$}\\
1 (an integer)\\
\textcolor{item}{$\bm{\{movie\_name\}}$}
\begin{itemize}[leftmargin=*]
\item Toy Story (1995)
\item Godfather, The (1972)
\item Small Wonders (1996)
\end{itemize}
\textcolor{item}{$\bm{\{recommended\_movies\}}$}
\begin{itemize}[leftmargin=*]
\item <- Austin Powers: International Man of Mystery (1997) -><- History ratings: 3.71 -> <- Summary: A groovy British spy travels back in time to stop his arch-nemesis from stealing his mojo. ->
\item <- Get Shorty (1995) -> <- History ratings: 3.62 -> <- Summary: A smooth-talking mobster turned Hollywood producer finds himself caught in a web of crime and comedy. ->
\item <- Full Monty, The (1997) -> <- History ratings: 3.87 -> <- Summary: A group of unemployed steelworkers decide to become male strippers to make ends meet. ->
\item <- Being John Malkovich (1999) -> <- History ratings: 4.13 -> <- Summary: A puppeteer discovers a portal that leads into the mind of actor John Malkovich. ->
\end{itemize}
\end{tcolorbox}

\begin{tcolorbox}[colback=background_e,colframe=frame_e,boxrule=0.5pt,title={\textbf{User Reaction Examples}}, enhanced, breakable]
% \textbf{Taste Generation}\\
\textbf{User Reaction to Recommended Items}
\begin{itemize}[leftmargin=*]
\item \textbf{Assessing Recommended List}\\
MOVIE: Breakfast Club, The (1985); ALIGN: Yes; REASON: I enjoy classic films and this movie falls into that category.\\
MOVIE: Desperately Seeking Susan (1985); ALIGN: No; REASON: I am not particularly interested in movies about bored housewives.\\
MOVIE: Mary Poppins (1964); ALIGN: Yes; REASON: I have a fondness for musicals and this is a classic one.\\
MOVIE: Bull Durham (1988); ALIGN: No; REASON: I am not a fan of movies about baseball.\\
\textbf{Watching Movies}\\
NUM: 2; WATCH: Breakfast Club, The (1985), Mary Poppins (1964); REASON: These movies align with my taste and I want to explore different genres.\\
\textbf{Rating Movies}\\
MOVIE: Breakfast Club, The (1985); RATING: 4; FEELING: I really enjoyed the character development and the unexpected friendships in this movie.\\
MOVIE: Mary Poppins (1964); RATING: 5; FEELING: The music, the magic, and the heartwarming story made this movie a delight to watch.
\end{itemize}
\textbf{Satisfaction Reflection}
\begin{itemize}[leftmargin=*]
\item Satisfied with the recommender system as it has recommended movies that I enjoyed and rated highly.
\item Unsatisfied with the recommendation result because I disliked some of the movies recommended to me.
\end{itemize}
\textbf{User Making Next Decision}
\begin{itemize}[leftmargin=*]
\item POSITIVE: I enjoyed watching "Citizen Kane" and rated it a 4. The recommender system did a good job in suggesting this movie to me.\\
Fatigue level: Low\\
\text{[NEXT]}; Reason: I'm feeling positive about the recommender system and I'm not tired yet, so I'll continue browsing.
\item NEGATIVE: I disliked some of the movies recommended to me on page 1 and did not watch or rate others. This has left me unsatisfied with the recommendation result so far.\\
\text{[EXIT]}; Reason: I am unsatisfied with the recommendations and I am starting to feel tired.
\end{itemize}
\end{tcolorbox}

\begin{tcolorbox}[colback=background_e,colframe=frame_e,boxrule=0.5pt,title={\textbf{User Profile Example}}, enhanced, breakable]
\textbf{Profile of User 254}\\
\textbf{Unique Tastes}\\
TASTE: I enjoy action-comedy movies.\\
REASON: I rated movies like "Airplane II: The Sequel" and "Naked Gun: From the Files of Police Squad!" highly, which are known for their comedic elements combined with action-packed sequences.\\
TASTE: I appreciate historical comedies.\\
REASON: Movies like "History of the World: Part I" and "Victor/Victoria" received high ratings from me due to their comedic portrayal of historical events and settings.\\
TASTE: I have a preference for adventure films.\\
REASON: Movies such as "Blue Lagoon" and "Room with a View, A" received positive ratings from me because they offer adventurous storylines and take the viewers on exciting journeys.\\
TASTE: I enjoy crime thrillers.\\
REASON: Movies like "Midnight Run" and "Cop Land" received high ratings from me due to their intense and suspenseful portrayal of crime-related stories.\\
TASTE: I appreciate heartwarming dramas.\\
REASON: Movies like "Driving Miss Daisy" and "Parenthood" received high ratings from me because they offer emotional and touching storylines that resonate with me.\\
TASTE: I have a preference for biographical films.
REASON: Movies such as "Good Morning, Vietnam" and "Almost Famous" received positive ratings from me because they are based on real-life events and offer insights into the lives of notable individuals.\\
\textbf{Rating Tendency}\\
The user tends to give high ratings (above 3) to movies that fall into genres such as action-comedy, historical comedy, adventure, crime thriller, heartwarming drama, and biographical films.\\
The user tends to give low ratings (below 2) to movies that do not align with their preferred genres, such as movies in genres like romance, horror, science fiction, or fantasy.\\
\textbf{Social Traits}\\
\textbf{Activity}: An Occasional Viewer, seldom attracted by movie recommendations. Only curious about watching movies that strictly align the taste. The movie-watching habits are not very infrequent. And you tend to exit the recommender system if you have a few unsatisfied memories.\\
\textbf{Conformity}: A Balanced Evaluator who considers both historical ratings and personal preferences when giving ratings to movies. Sometimes give ratings that are different from historical rating.\\
\textbf{Diversity}: A Cinematic Trailblazer, a relentless seeker of the unique and the obscure in the world of movies. The movie choices are so diverse and avant-garde that they defy categorization.
\end{tcolorbox}
